# Supplementary material for: Bandit based Dynamic Candidate Edge Selection in Solving Traveling Salesman Problems
Source: arXiv:2505.15862 source file (2025-06-05)
Supplement: Supplementary file 1 [file 06-Appendix.tex]

\section{Appendix}
% Algorithms solving routing problems usually need to collect some high-quality candidate edges to guide the search directions, so as to reduce the search space and enhance the search efficiency. However, we observe that in many algorithms, such as the classical Lin-Kernighan-Helsgaun (LKH) algorithm for the famous Traveling Salesman Problem (TSP), the candidate edges are predetermined and hardly change during the search. Such a stereotypical solution may cause the algorithm to get trapped in local optima. To this end, we enlarge the candidate sets to give other promising edges a chance to be selected and propose to use multi-armed bandit models for the appropriate candidate edge selection in each iteration. The bandit model can help LKH select candidate edges smartly and find better solutions. We further apply the bandit method to LKH-3, an extension of LKH that can solve TSP variant problems efficiently. Extensive experiments show the excellent performance of our method on various TSP benchmarks, and our method can also significantly improve LKH-3 in typical TSP variants. 

% 总的说一下我们的附录有哪些需要介绍
In appendix, we will supply three parts of full and additional experimental materials in experiments in \ref{Exp}, which contain comparison of \name and LKH in \ref{main_exep}, ablation study in \ref{ablation_exp} and generalization evaluation on the Multi-Traveling Salesman Problem(MTSP) in \ref{MTSP} and present them detailly in sequence. All these experiments confirm the excellent effectiveness of \name.

% 这里要说明一下每列参数的意思！
Before discussing appendix, the meaning of each column in the table would be explained. Instance means the name of experimental example, BKS is a abbreviation of best known solution and Success means how many times did BKS be included in the total runs of a instance. Best and Average means the best solution and average solution respectively, represented by percentage numbers. The average trials times and runtime are showed by Trials and Time.

\subsection{Supplement of Comparison of \name and LKH}
% 说主实验大概在做什么，和正文的呼应一下,测试了哪些用例
In main experiments \ref{main_exep}, we compare LKH using $k$ equals to 5 with \name using $m$ equals to 4 and $C_{max}$ is 7, which achieve excellent results in Small and medium-sized instances and  competitive result in big instances. In order to further confirm the effectiveness of \name, considering limited space, we do a fair comparison between \name and LKH, using that $m$ equals to 5, $C_{max}$ is 7 and $k$ equals to 5. In addtition, the other parameters are unchanged. We test 104 instances including all instances in TSPLIB, which has 7 hard instances such as pla33810 and pla85900, 22 big instances more than 10000 cities and less than 30000 cities in National TSPs and VLSI TSPs.

\begin{table*}[h]
\centering
\footnotesize
\resizebox{\linewidth}{!}{
\begin{tabular}{rr|rrrrr|rrrrr}
\hline
\multicolumn{1}{l}{} & \multicolumn{1}{l}{} & \multicolumn{5}{c}{LKH}                                                & \multicolumn{5}{c}{\name}                               \\
Instance             & BKS                  & Success & Best(\%)          & Average(\%)         & Trials & Time(s)   & Success & Best(\%)          & Average(\%)         & Trials & Time(s)   \\ \hline
a280                 & 2579                 & 10/10   & \textbf{2579(0.0000)}     & \textbf{2579(0.0000)}      & 1      & 0.012     & 10/10   & \textbf{2579(0.0000)}      & \textbf{2579(0.0000)}        & 1.1    & 0.019     \\
ali535               & 202339               & 10/10   & \textbf{202339(0.0000)}   & \textbf{202339(0.0000)}    & 4.9    & 0.117     & 10/10   & \textbf{202339(0.0000)}    & \textbf{202339(0.0000)}      & 6.4    & 0.287     \\
att532               & 27686                & 10/10   & \textbf{27686(0.0000)}    & \textbf{27686(0.0000)}     & 71.2   & 0.417     & 10/10   & \textbf{27686(0.0000)}     & \textbf{27686(0.0000)}       & 22.9   & 1.062     \\
bier127              & 118282               & 10/10   & \textbf{118282(0.0000)}   & \textbf{118282(0.0000)}    & 1      & 0.006     & 10/10   & \textbf{118282(0.0000)}    & \textbf{118282(0.0000)}      & 1.1    & 0.011     \\
brg180               & 1950                 & 10/10   & \textbf{1950(0.0000)}     & \textbf{1950(0.0000)}      & 1.8    & 0.004     & 10/10   & \textbf{1950(0.0000)}      & \textbf{1950(0.0000)}        & 3      & 0.006     \\
ch130                & 6110                 & 10/10   & \textbf{6110(0.0000)}     & \textbf{6110(0.0000)}      & 2.6    & 0.011     & 10/10   & \textbf{6110(0.0000)}      & \textbf{6110(0.0000)}        & 1.3    & 0.01      \\
ch150                & 6528                 & 9/10    & \textbf{6528(0.0000)}     & 6528.5(0.0077)             & 60.1   & 0.045     & 10/10   & \textbf{6528(0.0000)}      & \textbf{6528(0.0000)}        & 23.3   & 0.082     \\
d1291                & 50801                & 5/10    & \textbf{50801(0.0000)}    & 50840(0.0768)              & 995.4  & 27.442    & 10/10   & \textbf{50801(0.0000)}     & \textbf{50801(0.0000)}       & 192.2  & 14.737    \\
d1655                & 62128                & 10/10   & \textbf{62128(0.0000)}    & \textbf{62128(0.0000)}     & 194.1  & 2.18      & 10/10   & \textbf{62128(0.0000)}     & \textbf{62128(0.0000)}       & 34.2   & 2.459     \\
d198                 & 15780                & 10/10   & \textbf{15780(0.0000)}    & \textbf{15780(0.0000)}     & 14     & 0.11      & 10/10   & \textbf{15780(0.0000)}     & \textbf{15780(0.0000)}       & 8.9    & 0.24      \\
d2103                & 80450                & 0/10    & 80471(0.0261)             & 80505.7(0.0692)            & 2103   & 67.067    & 7/10    & \textbf{80450(0.0000)}     & \textbf{80451(0.0012)}       & 1084   & 306.056   \\
d493                 & 35002                & 2/10    & \textbf{35002(0.0000)}    & 35003.6(0.0046)            & 419.3  & 2.615     & 10/10   & \textbf{35002(0.0000)}     & \textbf{35002(0.0000)}       & 28.2   & 0.976     \\
d657                 & 48912                & 10/10   & \textbf{48912(0.0000)}    & \textbf{48912(0.0000)}     & 46.2   & 0.277     & 10/10   & \textbf{48912(0.0000)}     & \textbf{48912(0.0000)}       & 20.9   & 0.539     \\
dsj1000              & 18660188             & 10/10   & \textbf{18660188(0.0000)} & \textbf{18660188(0.0000)}  & 366.8  & 6.738     & 10/10   & \textbf{18660188(0.0000)}  & \textbf{18660188(0.0000)}    & 87.5   & 14.936    \\
eil101               & 629                  & 10/10   & \textbf{629(0.0000)}      & \textbf{629(0.0000)}       & 1      & 0.005     & 10/10   & \textbf{629(0.0000)}       & \textbf{629(0.0000)}         & 1      & 0.006     \\
fl1400               & 20127                & 0/10    & 20164(0.1838)             & 20165.5(0.1913)            & 1400   & 113.295   & 6/10    & \textbf{20127(0.0000)}     & \textbf{20141.8(0.0735)}     & 721    & 219.178   \\
fl1577               & 22249                & 0/10    & 22254(0.0225)             & 22260.6(0.0521)            & 1577   & 1172.102  & 9/10    & \textbf{22249(0.0000)}     & \textbf{22249.5(0.0022)}     & 614.9  & 1920.794  \\
fl3795               & 28772                & 4/10    & \textbf{28772(0.0000)}    & 28783.2(0.0389)            & 2998.1 & 423.943   & 5/10    & \textbf{28772(0.0000)}     & \textbf{28778.5(0.0226)}     & 3012.3 & 2437.034  \\
fl417                & 11861                & 10/10   & \textbf{11861(0.0000)}    & \textbf{11861(0.0000)}     & 7.3    & 2.829     & 10/10   & \textbf{11861(0.0000)}     & \textbf{11861(0.0000)}       & 18.2   & 7.437     \\
fnl4461              & 182566               & 9/10    & \textbf{182566(0.0000)}   & 182566.5(0.0003)           & 923.1  & 31.053    & 10/10   & \textbf{182566(0.0000)}    & \textbf{182566(0.0000)}      & 153.4  & 37.022    \\
gil262               & 2378                 & 10/10   & \textbf{2378(0.0000)}     & \textbf{2378(0.0000)}      & 10.6   & 0.106     & 10/10   & \textbf{2378(0.0000)}      & \textbf{2378(0.0000)}        & 4.9    & 0.138     \\
gr120                & 6942                 & 10/10   & \textbf{6942(0.0000)}     & \textbf{6942(0.0000)}      & 1      & 0.006     & 10/10   & \textbf{6942(0.0000)}      & \textbf{6942(0.0000)}        & 1.6    & 0.01      \\
gr137                & 69853                & 10/10   & \textbf{69853(0.0000)}    & \textbf{69853(0.0000)}     & 1      & 0.008     & 9/10    & \textbf{69853(0.0000)}     & 69865.7(0.0182)              & 18.9   & 0.014     \\
gr202                & 40160                & 10/10   & \textbf{40160(0.0000)}    & \textbf{40160(0.0000)}     & 1      & 0.01      & 10/10   & \textbf{40160(0.0000)}     & \textbf{40160(0.0000)}       & 12.2   & 0.018     \\
gr229                & 134602               & 2/10    & \textbf{134602(0.0000)}   & 134613.2(0.0083)           & 203.1  & 0.204     & 10/10   & \textbf{134602(0.0000)}    & \textbf{134602(0.0000)}      & 25.9   & 0.142     \\
gr431                & 171414               & 3/10    & \textbf{171414(0.0000)}   & 171499.2(0.0497)           & 347    & 1.725     & 10/10   & \textbf{171414(0.0000)}    & \textbf{171414(0.0000)}      & 73.7   & 2.255     \\
gr666                & 294358               & 5/10    & \textbf{294358(0.0000)}   & 294417(0.0200)             & 459.8  & 2.413     & 6/10    & \textbf{294358(0.0000)}    & \textbf{294393.7(0.0121)}    & 372.9  & 10.014    \\
kroA150              & 26524                & 10/10   & \textbf{26524(0.0000)}    & \textbf{26524(0.0000)}     & 3.8    & 0.039     & 10/10   & \textbf{26524(0.0000)}     & \textbf{26524(0.0000)}       & 9.8    & 0.06      \\
kroA200              & 29368                & 10/10   & \textbf{29368(0.0000)}    & \textbf{29368(0.0000)}     & 1.7    & 0.05      & 10/10   & \textbf{29368(0.0000)}     & \textbf{29368(0.0000)}       & 4.4    & 0.11      \\
kroB150              & 26130                & 2/10    & \textbf{26130(0.0000)}    & 26131.6(0.0061)            & 128.4  & 0.244     & 10/10   & \textbf{26130(0.0000)}     & \textbf{26130(0.0000)}       & 54.1   & 0.212     \\
kroB200              & 29437                & 10/10   & \textbf{29437(0.0000)}    & \textbf{29437(0.0000)}     & 1      & 0.018     & 10/10   & \textbf{29437(0.0000)}     & \textbf{29437(0.0000)}       & 3.3    & 0.043     \\
lin105               & 14379                & 10/10   & \textbf{14379(0.0000)}    & \textbf{14379(0.0000)}     & 1      & 0.002     & 10/10   & \textbf{14379(0.0000)}     & \textbf{14379(0.0000)}       & 1      & 0.002     \\
lin318               & 42029                & 4/10    & \textbf{42029(0.0000)}    & 42085.4(0.1342)            & 249.3  & 0.551     & 9/10    & \textbf{42029(0.0000)}     & \textbf{42040.4(0.0271)}     & 53     & 0.34      \\
linhp318             & 41345                & 10/10   & \textbf{41345(0.0000)}    & \textbf{41345(0.0000)}     & 15     & 0.031     & 10/10   & \textbf{41345(0.0000)}     & \textbf{41345(0.0000)}       & 10.6   & 0.057     \\
nrw1379              & 56638                & 6/10    & \textbf{56638(0.0000)}    & 56640(0.0035)              & 759.3  & 8.867     & 6/10    & \textbf{56638(0.0000)}     & \textbf{56639.6(0.0028)}     & 928    & 35.265    \\
p654                 & 34643                & 10/10   & \textbf{34643(0.0000)}    & \textbf{34643(0.0000)}     & 22.9   & 7.778     & 10/10   & \textbf{34643(0.0000)}     & \textbf{34643(0.0000)}       & 19.6   & 17.493    \\
pa561                & 2763                 & 10/10   & \textbf{2763(0.0000)}     & \textbf{2763(0.0000)}      & 58.5   & 0.49      & 10/10   & \textbf{2763(0.0000)}      & \textbf{2763(0.0000)}        & 13.6   & 0.501     \\
pcb1173              & 56892                & 4/10    & \textbf{56892(0.0000)}    & 56895(0.0053)              & 844    & 3.922     & 8/10    & \textbf{56892(0.0000)}     & \textbf{56893(0.0018)}       & 418.4  & 9.791     \\
pcb3038              & 137694               & 4/10    & \textbf{137694(0.0000)}   & 137701.2(0.0052)           & 2078.6 & 69.555    & 5/10    & \textbf{137694(0.0000)}    & \textbf{137700.7(0.0049)}    & 2081.1 & 275.373   \\
pcb442               & 50778                & 10/10   & \textbf{50778(0.0000)}    & \textbf{50778(0.0000)}     & 8.2    & 0.134     & 10/10   & \textbf{50778(0.0000)}     & \textbf{50778(0.0000)}       & 10.8   & 0.225     \\
pla7397              & 23260728             & 10/10   & \textbf{23260728(0.0000)} & \textbf{23260728(0.0000)}  & 632.4  & 198.386   & 10/10   & \textbf{23260728(0.0000)}  & \textbf{23260728(0.0000)}    & 622.5  & 1005.701  \\
pr1002               & 259045               & 8/10    & \textbf{259045(0.0000)}   & 259045.6(0.0002)           & 549    & 3.131     & 10/10   & \textbf{259045(0.0000)}    & \textbf{259045(0.0000)}      & 90.7   & 2.83      \\
pr107                & 44303                & 10/10   & \textbf{44303(0.0000)}    & \textbf{44303(0.0000)}     & 1      & 0.081     & 10/10   & \textbf{44303(0.0000)}     & \textbf{44303(0.0000)}       & 1      & 0.41      \\
pr124                & 59030                & 10/10   & \textbf{59030(0.0000)}    & \textbf{59030(0.0000)}     & 1      & 0.031     & 10/10   & \textbf{59030(0.0000)}     & \textbf{59030(0.0000)}       & 1.3    & 0.062     \\
pr136                & 96772                & 10/10   & \textbf{96772(0.0000)}    & \textbf{96772(0.0000)}     & 1      & 0.058     & 10/10   & \textbf{96772(0.0000)}     & \textbf{96772(0.0000)}       & 1.9    & 0.184     \\
pr144                & 58537                & 10/10   & \textbf{58537(0.0000)}    & \textbf{58537(0.0000)}     & 1      & 0.259     & 10/10   & \textbf{58537(0.0000)}     & \textbf{58537(0.0000)}       & 1.5    & 0.595     \\
pr152                & 73682                & 10/10   & \textbf{73682(0.0000)}    & \textbf{73682(0.0000)}     & 29.4   & 0.485     & 10/10   & \textbf{73682(0.0000)}     & \textbf{73682(0.0000)}       & 35.6   & 4.086     \\
pr226                & 80369                & 10/10   & \textbf{80369(0.0000)}    & \textbf{80369(0.0000)}     & 1      & 0.057     & 10/10   & \textbf{80369(0.0000)}     & \textbf{80369(0.0000)}       & 7.9    & 0.303     \\
pr2392               & 378032               & 10/10   & \textbf{378032(0.0000)}   & \textbf{378032(0.0000)}    & 5.8    & 0.999     & 10/10   & \textbf{378032(0.0000)}    & \textbf{378032(0.0000)}      & 19     & 31.332    \\
pr299                & 48191                & 9/10    & \textbf{48191(0.0000)}    & 48194.3(0.0068)            & 51.7   & 0.362     & 10/10   & \textbf{48191(0.0000)}     & \textbf{48191(0.0000)}       & 21.6   & 0.682     \\
pr439                & 107217               & 10/10   & \textbf{107217(0.0000)}   & \textbf{107217(0.0000)}    & 39.5   & 0.504     & 10/10   & \textbf{107217(0.0000)}    & \textbf{107217(0.0000)}      & 56.7   & 1.407     \\ \hline
\end{tabular}
}
\caption{The first part of full supplement results of LKH and \name in main experiments. The best results appear in \bf{bold}. }
\label{appendix_main1}
\end{table*}
\begin{table*}[h]
\centering
\footnotesize
\resizebox{\linewidth}{!}{
\begin{tabular}{rr|rrrrr|rrrrr}
\hline
\multicolumn{1}{l}{} & \multicolumn{1}{l}{} & \multicolumn{5}{c}{LKH}                                                & \multicolumn{5}{c}{\name}                               \\
Instance             & BKS                  & Success & Best(\%)          & Average(\%)         & Trials & Time(s)   & Success & Best(\%)          & Average(\%)         & Trials & Time(s)   \\ \hline
rat195               & 2323                 & 9/10    & \textbf{2323(0.0000)}     & 2323.5(0.0215)             & 55     & 0.154     & 10/10   & \textbf{2323(0.0000)}      & \textbf{2323(0.0000)}        & 14.8   & 0.193     \\
rat575               & 6773                 & 2/10    & \textbf{6773(0.0000)}     & 6773.8(0.0118)             & 526.9  & 2.315     & 6/10    & \textbf{6773(0.0000)}      & \textbf{6773.4(0.0059)}      & 392.5  & 4.933     \\
rat783               & 8806                 & 10/10   & \textbf{8806(0.0000)}     & \textbf{8806(0.0000)}      & 4.2    & 0.106     & 10/10   & \textbf{8806(0.0000)}      & \textbf{8806(0.0000)}        & 8.4    & 0.284     \\
rd400                & 15281                & 10/10   & \textbf{15281(0.0000)}    & \textbf{15281(0.0000)}     & 33     & 0.227     & 10/10   & \textbf{15281(0.0000)}     & \textbf{15281(0.0000)}       & 10.1   & 0.271     \\
rl1304               & 252948               & 3/10    & \textbf{252948(0.0000)}   & 253156.4(0.0824)           & 1170   & 12.483    & 10/10   & \textbf{252948(0.0000)}    & \textbf{252948(0.0000)}      & 572.1  & 27.382    \\
rl1323               & 270199               & 6/10    & \textbf{270199(0.0000)}   & 270219.6(0.0076)           & 718.8  & 9.632     & 8/10    & \textbf{270199(0.0000)}    & \textbf{270204.4(0.0020)}    & 576.9  & 23.749    \\
rl1889               & 316536               & 0/10    & 316549(0.0041)            & 316549.8(0.0044)           & 1889   & 61.404    & 10/10   & \textbf{316536(0.0000)}    & \textbf{316536(0.0000)}      & 236.5  & 35.557    \\
rl5915               & 565530               & 1/10    & \textbf{565530(0.0000)}   & 565621.5(0.0162)           & 5915   & 242.045   & 3/10    & \textbf{565530(0.0000)}    & \textbf{565564.4(0.0061)}    & 4863.8 & 1663.582  \\
rl5934               & 556045               & 0/10    & 556172(0.0228)            & 556377.6(0.0598)           & 5934   & 305.024   & 8/10    & \textbf{556045(0.0000)}    & \textbf{556063.2(0.0033)}    & 3472.1 & 1607.182  \\
si1032               & 92650                & 10/10   & \textbf{92650(0.0000)}    & \textbf{92650(0.0000)}     & 152    & 22.711    & 10/10   & \textbf{92650(0.0000)}     & \textbf{92650(0.0000)}       & 34.7   & 48.224    \\
si175                & 21407                & 7/10    & \textbf{21407(0.0000)}    & 21407.3(0.0014)            & 105.9  & 6.151     & 9/10    & \textbf{21407(0.0000)}     & \textbf{21407.1(0.0005)}     & 35.3   & 4.947     \\
si535                & 48450                & 7/10    & \textbf{48450(0.0000)}    & 48451.1(0.0023)            & 311.6  & 21.276    & 9/10    & \textbf{48450(0.0000)}     & \textbf{48450.3(0.0006)}     & 138.9  & 31.976    \\
ts225                & 126643               & 10/10   & \textbf{126643(0.0000)}   & \textbf{126643(0.0000)}    & 1      & 0.037     & 10/10   & \textbf{126643(0.0000)}    & \textbf{126643(0.0000)}      & 1      & 0.054     \\
tsp225               & 3916                 & 10/10   & \textbf{3916(0.0000)}     & \textbf{3916(0.0000)}      & 1      & 0.043     & 10/10   & \textbf{3916(0.0000)}      & \textbf{3916(0.0000)}        & 2.4    & 0.068     \\
u1060                & 224094               & 5/10    & \textbf{224094(0.0000)}   & 224107.5(0.0060)           & 663.3  & 84.172    & 10/10   & \textbf{224094(0.0000)}    & \textbf{224094(0.0000)}      & 44.4   & 22.001    \\
u1432                & 152970               & 10/10   & \textbf{152970(0.0000)}   & \textbf{152970(0.0000)}    & 5.3    & 0.651     & 10/10   & \textbf{152970(0.0000)}    & \textbf{152970(0.0000)}      & 22.3   & 1.4       \\
u159                 & 42080                & 10/10   & \textbf{42080(0.0000)}    & \textbf{42080(0.0000)}     & 1      & 0.01      & 10/10   & \textbf{42080(0.0000)}     & \textbf{42080(0.0000)}       & 1      & 0.017     \\
u1817                & 57201                & 1/10    & \textbf{57201(0.0000)}    & 57251.1(0.0876)            & 1817   & 74.187    & 1/10    & \textbf{57201(0.0000)}     & \textbf{57237.3(0.0635)}     & 1750.3 & 260.667   \\
u2152                & 64253                & 3/10    & \textbf{64253(0.0000)}    & 64287.7(0.0540)            & 1614   & 73.809    & 8/10    & \textbf{64253(0.0000)}     & \textbf{64264.4(0.0177)}     & 793.6  & 135.393   \\
u2319                & 234256               & 10/10   & \textbf{234256(0.0000)}   & \textbf{234256(0.0000)}    & 3.1    & 1.091     & 10/10   & \textbf{234256(0.0000)}    & \textbf{234256(0.0000)}      & 15.8   & 5.271     \\
u574                 & 36905                & 10/10   & \textbf{36905(0.0000)}    & \textbf{36905(0.0000)}     & 149.9  & 0.965     & 10/10   & \textbf{36905(0.0000)}     & \textbf{36905(0.0000)}       & 12.7   & 0.552     \\
u724                 & 41910                & 10/10   & \textbf{41910(0.0000)}    & \textbf{41910(0.0000)}     & 125.4  & 1.779     & 10/10   & \textbf{41910(0.0000)}     & \textbf{41910(0.0000)}       & 80.3   & 2.894     \\
vm1084               & 239297               & 3/10    & \textbf{239297(0.0000)}   & 239372.6(0.0316)           & 824.1  & 32.982    & 8/10    & \textbf{239297(0.0000)}    & \textbf{239307.4(0.0043)}    & 323.9  & 26.508    \\
vm1748               & 336556               & 9/10    & \textbf{336556(0.0000)}   & 336557.3(0.0004)           & 1007.9 & 12.692    & 10/10   & \textbf{336556(0.0000)}    & \textbf{336556(0.0000)}      & 146.4  & 9.992     \\
bbz25234             & 69335                & 0/5     & 69343(0.0115)             & 69349.8(0.0213)            & 10000  & 2938.861  & 0/5     & \textbf{69340(0.0072)}     & \textbf{69346.2(0.0162)}     & 10000  & 21084.385 \\
brd14051             & 469385               & 0/5     & \textbf{469395(0.0021)}   & \textbf{469397.4(0.0026)}  & 10000  & 1789.55   & 0/5     & 469412(0.0058)             & 469460.6(0.0161)             & 10000  & 8240.87   \\
d15112               & 1573084              & 0/5     & \textbf{1573202(0.0075)}  & \textbf{1573242.6(0.0101)} & 10000  & 2109.107  & 0/5     & 1573288(0.0130)            & 1573318.8(0.0149)            & 10000  & 9560.618  \\
d18512               & 645238               & 0/5     & \textbf{645263(0.0039)}   & \textbf{645268.8(0.0048)}  & 10000  & 2668.676  & 0/5     & 645353(0.0178)             & 645424.4(0.0289)             & 10000  & 10513.633 \\
fi10639              & 520527               & 0/5     & \textbf{520534(0.0013)}   & \textbf{520562.8(0.0069)}  & 10000  & 844.409   & 0/5     & 520539(0.0023)             & 520564.2(0.0071)             & 10000  & 4636.342  \\
fma21553             & 66527                & 0/5     & 66529(0.0030)             & 66540.4(0.0201)            & 10000  & 2102.462  & 0/5     & \textbf{66527(0.0000)}     & \textbf{66534.8(0.0117)}     & 10000  & 11584.059 \\
fnc19402             & 59287                & 0/5     & 59303(0.0270)             & 59308.6(0.0364)            & 10000  & 1823.404  & 0/5     & \textbf{59295(0.0135)}     & \textbf{59298.6(0.0196)}     & 10000  & 9574.85   \\
frh19289             & 55798                & 0/5     & \textbf{55800(0.0036)}    & \textbf{55806.8(0.0158)}   & 10000  & 1836.776  & 0/5     & 55804(0.0108)              & 55808.8(0.0194)              & 10000  & 11312.593 \\
fyg28534             & 78562                & 0/5     & 78571(0.0115)             & 78574.6(0.0160)            & 10000  & 2941.719  & 0/5     & \textbf{78568(0.0076)}     & \textbf{78573.2(0.0143)}     & 10000  & 21597.032 \\
ho14473              & 177092               & 0/5     & 177161(0.0390)            & 177182.6(0.0512)           & 332.2  & 43362.256 & 0/5     & \textbf{177117(0.0141)}    & \textbf{177138(0.0260)}      & 402.8  & 43336.187 \\
icx28698             & 78087                & 0/5     & 78100(0.0166)             & 78106.8(0.0254)            & 10000  & 3237.22   & 0/5     & \textbf{78093(0.0077)}     & \textbf{78104.4(0.0223)}     & 10000  & 22079.871 \\
ido21215             & 63517                & 0/5     & 63525(0.0126)             & 63533.6(0.0261)            & 10000  & 2161.696  & 0/5     & \textbf{63519(0.0031)}     & \textbf{63525.6(0.0135)}     & 10000  & 14603.814 \\
ird29514             & 80353                & 0/5     & \textbf{80366(0.0162)}    & \textbf{80374.8(0.0271)}   & 10000  & 3052.619  & 0/5     & 80380(0.0336)              & 80392.4(0.0490)              & 10000  & 24177.144 \\
irx28268             & 72608                & 0/5     & 72614(0.0083)             & 72622(0.0193)              & 10000  & 2979.1    & 0/5     & \textbf{72608(0.0000)}     & \textbf{72610.2(0.0030)}     & 10000  & 17642.291 \\
it16862              & 557315               & 0/5     & \textbf{557319(0.0007)}   & 557336(0.0038)             & 10000  & 6012.144  & 0/5     & \textbf{557319(0.0007)}    & \textbf{557332.4(0.0031)}    & 8975   & 39870.583 \\
lsb22777             & 60977                & 0/5     & 60981(0.0066)             & 60989(0.0197)              & 10000  & 2625.606  & 0/5     & \textbf{60978(0.0016)}     & \textbf{60983.8(0.0112)}     & 10000  & 15632.943 \\
mo14185              & 427377               & 0/5     & 427381(0.0009)            & 427402.6(0.0060)           & 10000  & 1408.069  & 0/5     & \textbf{427380(0.0007)}    & \textbf{427385.8(0.0021)}    & 10000  & 6173.498  \\
pjh17845             & 48092                & 0/5     & \textbf{48093(0.0021)}    & 48100.4(0.0175)            & 10000  & 1739.081  & 0/5     & \textbf{48093(0.0021)}     & \textbf{48095.6(0.0075)}     & 10000  & 10022.941 \\
pla33810             & 66048945             & 0/5     & 66061689(0.0193)          & 66065656.2(0.0253)         & 3000   & 25030.561 & 0/5     & \textbf{66052269(0.0050)}  & \textbf{66062745(0.0209)}    & 1442.4 & 29411.211 \\
pla85900             & 142382641            & 0/5     & 142455345(0.0511)         & 142457070.8(0.0523)        & 3000   & 9270.294  & 0/5     & \textbf{142404864(0.0156)} & \textbf{142411899.2(0.0205)} & 3000   & 25842.528 \\
rl11849              & 923288               & 0/5     & \textbf{923288(0.0000)}   & 923360.2(0.0078)           & 9257.4 & 947.406   & 0/5     & \textbf{923288(0.0000)}    & \textbf{923323.6(0.0039)}    & 8532   & 3633.087  \\
sw24978              & 855597               & 0/5     & 855599(0.0002)            & 855628(0.0036)             & 10000  & 2807.107  & 0/5     & \textbf{855602(0.0006)}    & \textbf{855611.8(0.0017)}    & 10000  & 17463.642 \\
usa13509             & 19982859             & 0/5     & \textbf{19982874(0.0001)} & 19983306.2(0.0022)         & 10000  & 1111.746  & 0/5     & 19983027(0.0008)           & \textbf{19983277.2(0.0021)}  & 10000  & 6300.91   \\
vm22775              & 569288               & 0/5     & 569299(0.0019)            & \textbf{569308.6(0.0036)}  & 10000  & 7171.503  & 0/5     & \textbf{569290(0.0004)}    & 569308.8(0.0037)             & 10000  & 20219.204 \\
xia16928             & 52850                & 0/5     & \textbf{52850(0.0000)}    & 52853.2(0.0061)            & 10000  & 1673.976  & 0/5     & \textbf{52850(0.0000)}     & \textbf{52852(0.0038)}       & 10000  & 9295.233  \\
xmc10150             & 28387                & 0/5     & \textbf{28388(0.0035)}    & \textbf{28388.8(0.0063)}   & 10000  & 832.771   & 0/5     & 28389(0.0070)              & 28390.8(0.0134)              & 10000  & 4279.319  \\
xrb14233             & 45462                & 0/5     & 45466(0.0088)             & 45468.4(0.0141)            & 10000  & 1376.691  & 0/5     & \textbf{45462(0.0000)}     & \textbf{45465(0.0066)}       & 10000  & 6659.296  \\
xrh24104             & 69294                & 0/5     & 69300(0.0087)             & 69304.2(0.0147)            & 10000  & 2303.957  & 0/5     & \textbf{69297(0.0043)}     & \textbf{69303.2(0.0133)}     & 10000  & 16508.957 \\
xvb13584             & 37083                & 0/5     & \textbf{37083(0.0000)}    & \textbf{37087.2(0.0113)}   & 8251.2 & 1053.738  & 0/5     & 37086(0.0081)              & 37090.4(0.0200)              & 10000  & 5740.314  \\ \hline
                     & Average Gap(\%)      &         & 0.0051                    & 0.0149                     &        &           &         & 0.0018                     & 0.0064                       &        &          \\ \hline
\end{tabular}
}
\caption{The second part of full supplement results of LKH and \name in main experiments. The best results appear in \bf{bold}. }
\label{appendix_main2}
\end{table*}

% 实验表明
As shown in the table \ref{appendix_main1} and \ref{appendix_main2}, the proposed method make great progress based on LKH. The average gap counted by all 104 instances in Best and Average column is 0.0018\% and 0.0064\% which are smaller than 0.0051\% and 0.0149\% in LKH. Noted that, among 29 big instances, \name obtains a better result than LKH in 16 (resp. 20) instances in terms of the best (resp. average) solutions and a worse result than LKH in 2 (resp. 9) instances in terms of the best (resp. average) solutions. As for small and medium-sized instances, \name has absolute preference for LKH.

% 分析一下七选四和七选五，最后说我们的算法好
In section \ref{main_exep}, \name only use 4 original default edges rather than 5 to join in local search, making competitive outcome for LKH. When we enlarge $m$ to 5 in MAB model which equals to $k$ in LKH, it makes geat progress based relative to LKH. Generally speaking, \name can provide more high quality and suitable edges $k$-opt operation, which shows the effectiveness of our method.

\subsection{Supplement of Ablation}

To verify effectiveness of our proposed method, we did two ablation experiments, called ablation study on the arm selection strategy study and the MAB model, which will be divided into two subsection to talk about in sequence. 75 instances in TSPLIB less than 10000 cities are tested below and all parameters are same as main experiments in \ref{main_exep}.

\subsubsection{Full Results of Ablation Study on the Arm Selection Strategy}
% 实验表明，缺一不可
In this section, we supply full result of the arm selection strategy to show our the design in MAB model is reasonable. Table \ref{append_epsilon} include all results using the arm selection stratege without $\epsilon$-greedy, table \ref{appendix_M} without $M$-greedy and table \ref{appendix_alpha} without $\alpha$-greedy.

\begin{table*}[h]
\centering
\footnotesize
\resizebox{\linewidth}{!}{
% Please add the following required packages to your document preamble:
% \usepackage{multirow}
% Please add the following required packages to your document preamble:
% \usepackage{multirow}
\begin{tabular}{rr|rrrrr|rrrrr}
\hline
\multicolumn{1}{l}{} & \multicolumn{1}{l}{} & \multicolumn{5}{c}{\name}                                                   & \multicolumn{5}{c}{\name-no$\epsilon$}                                      \\
Instance             & BKS                  & Success        & Best(\%)                  & Average(\%)               & Trials & Time(s)  & Success        & Best(\%)                  & Average(\%)               & Trials & Time(s)  \\ \hline
a280                 & 2579                 & \textbf{10/10} & \textbf{2579(0.0000)}     & \textbf{2579(0.0000)}     & 2.4    & 0.025    & \textbf{10/10} & \textbf{2579(0.0000)}     & \textbf{2579(0.0000)}     & 1      & 0.017    \\
ali535               & 202339               & \textbf{10/10} & \textbf{202339(0.0000)}   & \textbf{202339(0.0000)}   & 4.2    & 0.325    & \textbf{10/10} & \textbf{202339(0.0000)}   & \textbf{202339(0.0000)}   & 2.8    & 0.182    \\
att532               & 27686                & \textbf{10/10} & \textbf{27686(0.0000)}    & \textbf{27686(0.0000)}    & 29.2   & 1.597    & \textbf{10/10} & \textbf{27686(0.0000)}    & \textbf{27686(0.0000)}    & 61.9   & 1.482    \\
bier127              & 118282               & \textbf{10/10} & \textbf{118282(0.0000)}   & \textbf{118282(0.0000)}   & 1.9    & 0.019    & \textbf{10/10} & \textbf{118282(0.0000)}   & \textbf{118282(0.0000)}   & 1      & 0.01     \\
brg180               & 1950                 & \textbf{10/10} & \textbf{1950(0.0000)}     & \textbf{1950(0.0000)}     & 3.9    & 0.006    & \textbf{10/10} & \textbf{1950(0.0000)}     & \textbf{1950(0.0000)}     & 5.3    & 0.007    \\
ch130                & 6110                 & \textbf{10/10} & \textbf{6110(0.0000)}     & \textbf{6110(0.0000)}     & 4      & 0.017    & \textbf{10/10} & \textbf{6110(0.0000)}     & \textbf{6110(0.0000)}     & 1      & 0.009    \\
ch150                & 6528                 & \textbf{10/10} & \textbf{6528(0.0000)}     & \textbf{6528(0.0000)}     & 27.3   & 0.056    & \textbf{10/10} & \textbf{6528(0.0000)}     & \textbf{6528(0.0000)}     & 18.4   & 0.052    \\
d1291                & 50801                & \textbf{10/10} & \textbf{50801(0.0000)}    & \textbf{50801(0.0000)}    & 170.1  & 16.348   & \textbf{10/10} & \textbf{50801(0.0000)}    & \textbf{50801(0.0000)}    & 131.7  & 6.12     \\
d1655                & 62128                & \textbf{10/10} & \textbf{62128(0.0000)}    & \textbf{62128(0.0000)}    & 39.3   & 1.108    & \textbf{10/10} & \textbf{62128(0.0000)}    & \textbf{62128(0.0000)}    & 41.4   & 2.062    \\
d198                 & 15780                & \textbf{10/10} & \textbf{15780(0.0000)}    & \textbf{15780(0.0000)}    & 18.3   & 0.454    & \textbf{10/10} & \textbf{15780(0.0000)}    & \textbf{15780(0.0000)}    & 16.3   & 0.281    \\
d2103                & 80450                & \textbf{6/10}  & \textbf{80450(0.0000)}    & \textbf{80451.5(0.0019)}  & 945.7  & 474.485  & \textbf{3/10}  & \textbf{80450(0.0000)}    & \textbf{80452.6(0.0032)}  & 1742.5 & 296.101  \\
d493                 & 35002                & \textbf{10/10} & \textbf{35002(0.0000)}    & \textbf{35002(0.0000)}    & 50.7   & 1.687    & \textbf{10/10} & \textbf{35002(0.0000)}    & \textbf{35002(0.0000)}    & 9.9    & 0.296    \\
d657                 & 48912                & \textbf{10/10} & \textbf{48912(0.0000)}    & \textbf{48912(0.0000)}    & 25.7   & 0.673    & \textbf{10/10} & \textbf{48912(0.0000)}    & \textbf{48912(0.0000)}    & 42.9   & 0.603    \\
dsj1000              & 18660188             & \textbf{10/10} & \textbf{18660188(0.0000)} & \textbf{18660188(0.0000)} & 31     & 9.069    & \textbf{10/10} & \textbf{18660188(0.0000)} & \textbf{18660188(0.0000)} & 58.5   & 7.471    \\
eil101               & 629                  & \textbf{10/10} & \textbf{629(0.0000)}      & \textbf{629(0.0000)}      & 1      & 0.005    & \textbf{10/10} & \textbf{629(0.0000)}      & \textbf{629(0.0000)}      & 1      & 0.005    \\
fl1400               & 20127                & \textbf{3/10}  & \textbf{20127(0.0000)}    & \textbf{20152.9(0.1287)}  & 1115.4 & 426.471  & 1/10           & \textbf{20127(0.0000)}    & 20160.3(0.1654)           & 1316.1 & 238.621  \\
fl1577               & 22249                & \textbf{10/10} & \textbf{22249(0.0000)}    & \textbf{22249(0.0000)}    & 303.5  & 3112.618 & \textbf{8/10}  & \textbf{22249(0.0000)}    & \textbf{22250.7(0.0076)}  & 471.2  & 1384.166 \\
fl3795               & 28772                & \textbf{4/10}  & \textbf{28772(0.0000)}    & \textbf{28779.8(0.0271)}  & 2590.4 & 2379.836 & \textbf{8/10}  & \textbf{28772(0.0000)}    & \textbf{28774.6(0.0090)}  & 1649.1 & 636.055  \\
fl417                & 11861                & \textbf{10/10} & \textbf{11861(0.0000)}    & \textbf{11861(0.0000)}    & 7.2    & 13.871   & \textbf{10/10} & \textbf{11861(0.0000)}    & \textbf{11861(0.0000)}    & 9.5    & 5.74     \\
fnl4461              & 182566               & \textbf{10/10} & \textbf{182566(0.0000)}   & \textbf{182566(0.0000)}   & 322.4  & 74.652   & \textbf{10/10} & \textbf{182566(0.0000)}   & \textbf{182566(0.0000)}   & 216.5  & 29.921   \\
gil262               & 2378                 & \textbf{10/10} & \textbf{2378(0.0000)}     & \textbf{2378(0.0000)}     & 7      & 0.247    & \textbf{10/10} & \textbf{2378(0.0000)}     & \textbf{2378(0.0000)}     & 11.6   & 0.172    \\
gr120                & 6942                 & \textbf{10/10} & \textbf{6942(0.0000)}     & \textbf{6942(0.0000)}     & 4.5    & 0.009    & \textbf{10/10} & \textbf{6942(0.0000)}     & \textbf{6942(0.0000)}     & 1      & 0.007    \\
gr137                & 69853                & 9/10           & \textbf{69853(0.0000)}    & 69865.7(0.0182)           & 14.6   & 0.024    & \textbf{10/10} & \textbf{69853(0.0000)}    & \textbf{69853(0.0000)}    & 1.3    & 0.012    \\
gr202                & 40160                & \textbf{10/10} & \textbf{40160(0.0000)}    & \textbf{40160(0.0000)}    & 2.4    & 0.029    & \textbf{10/10} & \textbf{40160(0.0000)}    & \textbf{40160(0.0000)}    & 3.7    & 0.014    \\
gr229                & 134602               & \textbf{10/10} & \textbf{134602(0.0000)}   & \textbf{134602(0.0000)}   & 22     & 0.096    & \textbf{10/10} & \textbf{134602(0.0000)}   & \textbf{134602(0.0000)}   & 9.3    & 0.074    \\
gr431                & 171414               & \textbf{10/10} & \textbf{171414(0.0000)}   & \textbf{171414(0.0000)}   & 107    & 2.997    & \textbf{9/10}  & \textbf{171414(0.0000)}   & \textbf{171414.2(0.0001)} & 195.9  & 4.378    \\
gr666                & 294358               & 7/10           & \textbf{294358(0.0000)}   & 294393.4(0.0120)          & 372.4  & 9.903    & \textbf{9/10}  & \textbf{294358(0.0000)}   & \textbf{294369.8(0.0040)} & 293.1  & 6.281    \\
kroA150              & 26524                & \textbf{10/10} & \textbf{26524(0.0000)}    & \textbf{26524(0.0000)}    & 2.3    & 0.074    & \textbf{10/10} & \textbf{26524(0.0000)}    & \textbf{26524(0.0000)}    & 1.4    & 0.045    \\
kroA200              & 29368                & \textbf{10/10} & \textbf{29368(0.0000)}    & \textbf{29368(0.0000)}    & 2.5    & 0.156    & \textbf{10/10} & \textbf{29368(0.0000)}    & \textbf{29368(0.0000)}    & 2      & 0.105    \\
kroB150              & 26130                & \textbf{8/10}  & \textbf{26130(0.0000)}    & \textbf{26130.4(0.0015)}  & 51.7   & 0.222    & 5/10           & \textbf{26130(0.0000)}    & 26131(0.0038)             & 119.5  & 0.299    \\
kroB200              & 29437                & \textbf{10/10} & \textbf{29437(0.0000)}    & \textbf{29437(0.0000)}    & 2.1    & 0.067    & \textbf{9/10}  & \textbf{29437(0.0000)}    & \textbf{29441.2(0.0143)}  & 30.1   & 0.075    \\
lin105               & 14379                & \textbf{10/10} & \textbf{14379(0.0000)}    & \textbf{14379(0.0000)}    & 1      & 0.002    & \textbf{10/10} & \textbf{14379(0.0000)}    & \textbf{14379(0.0000)}    & 1      & 0.002    \\
lin318               & 42029                & \textbf{8/10}  & \textbf{42029(0.0000)}    & \textbf{42051.8(0.0542)}  & 140.8  & 0.525    & 10/10          & \textbf{41345(0.0000)}    & \textbf{41345(0.0000)}    & 19.2   & 0.073    \\
lin318               & 41345                & \textbf{10/10} & \textbf{41345(0.0000)}    & \textbf{41345(0.0000)}    & 16.7   & 0.087    & \textbf{4/10}  & \textbf{42029(0.0000)}    & \textbf{42097.4(0.1627)}  & 219.1  & 0.429    \\
nrw1379              & 56638                & \textbf{10/10} & \textbf{56638(0.0000)}    & \textbf{56638(0.0000)}    & 476.9  & 23.146   & 10/10          & \textbf{56638(0.0000)}    & \textbf{56638(0.0000)}    & 447.9  & 11.767   \\
p654                 & 34643                & \textbf{10/10} & \textbf{34643(0.0000)}    & \textbf{34643(0.0000)}    & 15.6   & 45.578   & \textbf{10/10} & \textbf{34643(0.0000)}    & \textbf{34643(0.0000)}    & 18.5   & 7.997    \\
pa561.tsp            & 2763                 & \textbf{10/10} & \textbf{2763(0.0000)}     & \textbf{2763(0.0000)}     & 13.7   & 0.81     & \textbf{10/10} & \textbf{2763(0.0000)}     & \textbf{2763(0.0000)}     & 13.5   & 0.453    \\
pcb1173              & 56892                & \textbf{6/10}  & \textbf{56892(0.0000)}    & \textbf{56894(0.0035)}    & 721.2  & 15.051   & \textbf{4/10}  & \textbf{56892(0.0000)}    & \textbf{56895(0.0053)}    & 903    & 12.673   \\
pcb3038              & 137694               & \textbf{9/10}  & \textbf{137694(0.0000)}   & \textbf{137694.5(0.0004)} & 1021.9 & 167.493  & \textbf{9/10}  & \textbf{137694(0.0000)}   & \textbf{137694.6(0.0004)} & 794.8  & 86.537   \\
pcb442               & 50778                & \textbf{10/10} & \textbf{50778(0.0000)}    & \textbf{50778(0.0000)}    & 4.8    & 0.185    & \textbf{10/10} & \textbf{50778(0.0000)}    & \textbf{50778(0.0000)}    & 4.8    & 0.134    \\
pla7397              & 23260728             & \textbf{10/10} & \textbf{23260728(0.0000)} & \textbf{23260728(0.0000)} & 206.4  & 889.849  & \textbf{10/10} & \textbf{23260728(0.0000)} & \textbf{23260728(0.0000)} & 906.7  & 807.784  \\
pr1002               & 259045               & \textbf{10/10} & \textbf{259045(0.0000)}   & \textbf{259045(0.0000)}   & 281.1  & 4.893    & \textbf{10/10} & \textbf{259045(0.0000)}   & \textbf{259045(0.0000)}   & 92.2   & 1.928    \\
pr107                & 44303                & \textbf{10/10} & \textbf{44303(0.0000)}    & \textbf{44303(0.0000)}    & 1.7    & 0.106    & \textbf{10/10} & \textbf{44303(0.0000)}    & \textbf{44303(0.0000)}    & 1      & 0.175    \\
pr124                & 59030                & \textbf{10/10} & \textbf{59030(0.0000)}    & \textbf{59030(0.0000)}    & 2.2    & 0.03     & \textbf{10/10} & \textbf{59030(0.0000)}    & \textbf{59030(0.0000)}    & 1      & 0.075    \\
pr136                & 96772                & \textbf{10/10} & \textbf{96772(0.0000)}    & \textbf{96772(0.0000)}    & 1.8    & 0.314    & \textbf{10/10} & \textbf{96772(0.0000)}    & \textbf{96772(0.0000)}    & 1      & 0.113    \\
pr144                & 58537                & \textbf{10/10} & \textbf{58537(0.0000)}    & \textbf{58537(0.0000)}    & 2.9    & 0.98     & \textbf{10/10} & \textbf{58537(0.0000)}    & \textbf{58537(0.0000)}    & 1      & 1.146    \\
pr152                & 73682                & \textbf{10/10} & \textbf{73682(0.0000)}    & \textbf{73682(0.0000)}    & 9.7    & 3.531    & \textbf{9/10}  & \textbf{73682(0.0000)}    & \textbf{73695.6(0.0185)}  & 46.7   & 1.032    \\
pr226                & 80369                & \textbf{10/10} & \textbf{80369(0.0000)}    & \textbf{80369(0.0000)}    & 12.4   & 0.591    & \textbf{10/10} & \textbf{80369(0.0000)}    & \textbf{80369(0.0000)}    & 1.8    & 0.151    \\
pr2392               & 378032               & \textbf{10/10} & \textbf{378032(0.0000)}   & \textbf{378032(0.0000)}   & 13.3   & 42.932   & \textbf{10/10} & \textbf{378032(0.0000)}   & \textbf{378032(0.0000)}   & 22.4   & 29.641   \\
pr299                & 48191                & \textbf{10/10} & \textbf{48191(0.0000)}    & \textbf{48191(0.0000)}    & 3.3    & 0.488    & \textbf{10/10} & \textbf{48191(0.0000)}    & \textbf{48191(0.0000)}    & 2.3    & 0.203    \\
pr439                & 107217               & \textbf{10/10} & \textbf{107217(0.0000)}   & \textbf{107217(0.0000)}   & 65.1   & 1.86     & \textbf{10/10} & \textbf{107217(0.0000)}   & \textbf{107217(0.0000)}   & 37.7   & 0.682    \\
rat195               & 2323                 & \textbf{10/10} & \textbf{2323(0.0000)}     & \textbf{2323(0.0000)}     & 24.7   & 0.285    & \textbf{10/10} & \textbf{2323(0.0000)}     & \textbf{2323(0.0000)}     & 13.2   & 0.167    \\
rat575               & 6773                 & \textbf{7/10}  & \textbf{6773(0.0000)}     & \textbf{6773.4(0.0059)}   & 286.9  & 3.388    & 3/10           & \textbf{6773(0.0000)}     & 6773.7(0.0103)            & 442.1  & 3.465    \\
rat783               & 8806                 & \textbf{10/10} & \textbf{8806(0.0000)}     & \textbf{8806(0.0000)}     & 18.4   & 0.595    & \textbf{10/10} & \textbf{8806(0.0000)}     & \textbf{8806(0.0000)}     & 17.2   & 0.273    \\
rd400                & 15281                & \textbf{10/10} & \textbf{15281(0.0000)}    & \textbf{15281(0.0000)}    & 34     & 0.534    & \textbf{10/10} & \textbf{15281(0.0000)}    & \textbf{15281(0.0000)}    & 21.5   & 0.24     \\
rl1304               & 252948               & \textbf{8/10}  & \textbf{252948(0.0000)}   & 252991.3(0.0171)          & 493.4  & 19.742   & \textbf{7/10}  & \textbf{252948(0.0000)}   & \textbf{252963.3(0.0060)} & 804.3  & 18.261   \\
rl1323               & 270199               & \textbf{9/10}  & \textbf{270199(0.0000)}   & \textbf{270201.7(0.0010)} & 358.2  & 18.002   & \textbf{7/10}  & \textbf{270199(0.0000)}   & \textbf{270207.1(0.0030)} & 554.3  & 12.731   \\
rl1889               & 316536               & \textbf{10/10} & \textbf{316536(0.0000)}   & \textbf{316536(0.0000)}   & 420.2  & 91.595   & 9/10           & \textbf{316536(0.0000)}   & 316546.2(0.0032)          & 583.7  & 46.735   \\
rl5915               & 565530               & \textbf{2/10}  & \textbf{565530(0.0000)}   & \textbf{565573.3(0.0077)} & 4927.6 & 1521.327 & \textbf{1/10}  & \textbf{565530(0.0000)}   & \textbf{565578.8(0.0086)} & 5915   & 1160.764 \\
rl5934               & 556045               & \textbf{5/10}  & \textbf{556045(0.0000)}   & \textbf{556130.2(0.0153)} & 4207.3 & 2004.291 & \textbf{0/10}  & \textbf{556136(0.0164)}   & \textbf{556144.3(0.0179)} & 5934   & 1869.455 \\
si1032               & 92650                & \textbf{10/10} & \textbf{92650(0.0000)}    & \textbf{92650(0.0000)}    & 15.5   & 87.295   & \textbf{10/10} & \textbf{92650(0.0000)}    & \textbf{92650(0.0000)}    & 73.4   & 38.228   \\
si175                & 21407                & 7/10           & \textbf{21407(0.0000)}    & 21407.3(0.0014)           & 69.2   & 8.273    & \textbf{10/10} & \textbf{21407(0.0000)}    & \textbf{21407(0.0000)}    & 28.7   & 2.275    \\
si535                & 48450                & \textbf{8/10}  & \textbf{48450(0.0000)}    & \textbf{48450.6(0.0012)}  & 192.8  & 77.812   & \textbf{10/10} & \textbf{48450(0.0000)}    & \textbf{48450(0.0000)}    & 127.9  & 15.046   \\
ts225                & 126643               & \textbf{10/10} & \textbf{126643(0.0000)}   & \textbf{126643(0.0000)}   & 1      & 0.027    & \textbf{10/10} & \textbf{126643(0.0000)}   & \textbf{126643(0.0000)}   & 1      & 0.044    \\
tsp225               & 3916                 & \textbf{10/10} & \textbf{3916(0.0000)}     & \textbf{3916(0.0000)}     & 3.5    & 0.132    & \textbf{10/10} & \textbf{3916(0.0000)}     & \textbf{3916(0.0000)}     & 1      & 0.074    \\
u1060                & 224094               & \textbf{10/10} & \textbf{224094(0.0000)}   & \textbf{224094(0.0000)}   & 113.1  & 113.18   & \textbf{10/10} & \textbf{224094(0.0000)}   & \textbf{224094(0.0000)}   & 34.5   & 10.792   \\
u1432                & 152970               & \textbf{10/10} & \textbf{152970(0.0000)}   & \textbf{152970(0.0000)}   & 9.5    & 1.325    & \textbf{10/10} & \textbf{152970(0.0000)}   & \textbf{152970(0.0000)}   & 9.5    & 1.145    \\
u159                 & 42080                & \textbf{10/10} & \textbf{42080(0.0000)}    & \textbf{42080(0.0000)}    & 2.8    & 0.017    & \textbf{10/10} & \textbf{42080(0.0000)}    & \textbf{42080(0.0000)}    & 1      & 0.013    \\
u1817                & 57201                & \textbf{0/10}  & \textbf{57216(0.0262)}    & \textbf{57242.3(0.0722)}  & 1817   & 481.484  & \textbf{0/10}  & \textbf{57225(0.0420)}    & \textbf{57243.9(0.0750)}  & 1817   & 231.217  \\
u2152                & 64253                & \textbf{9/10}  & \textbf{64253(0.0000)}    & \textbf{64257(0.0062)}    & 800.9  & 160.547  & \textbf{9/10}  & \textbf{64253(0.0000)}    & \textbf{64257(0.0062)}    & 805.3  & 84.169   \\
u2319                & 234256               & \textbf{10/10} & \textbf{234256(0.0000)}   & \textbf{234256(0.0000)}   & 17.8   & 6.453    & \textbf{10/10} & \textbf{234256(0.0000)}   & \textbf{234256(0.0000)}   & 4.3    & 1.74     \\
u574                 & 36905                & \textbf{10/10} & \textbf{36905(0.0000)}    & \textbf{36905(0.0000)}    & 33     & 1.126    & \textbf{10/10} & \textbf{36905(0.0000)}    & \textbf{36905(0.0000)}    & 2.2    & 0.214    \\
u724                 & 41910                & \textbf{10/10} & \textbf{41910(0.0000)}    & \textbf{41910(0.0000)}    & 90.6   & 3.3      & \textbf{10/10} & \textbf{41910(0.0000)}    & \textbf{41910(0.0000)}    & 92.1   & 2.638    \\
vm1084               & 239297               & \textbf{8/10}  & \textbf{239297(0.0000)}   & \textbf{239307.4(0.0043)} & 419.8  & 51.722   & \textbf{8/10}  & \textbf{239297(0.0000)}   & \textbf{239309.9(0.0054)} & 324.8  & 17.299   \\
vm1748               & 336556               & \textbf{10/10} & \textbf{336556(0.0000)}   & \textbf{336556(0.0000)}   & 257.7  & 18.207   & \textbf{9/10}  & \textbf{336556(0.0000)}   & \textbf{336570.5(0.0043)} & 620.3  & 28.457   \\ \hline
                     & Average Gap(\%)      &                & \textbf{0.0003}           & \textbf{0.0051}           &        &          &                & 0.0008                    & 0.0071                    &        &     \\ \hline    
\end{tabular}
}
\caption{Full comparisonal results of \name-no$\epsilon$ and \name in ablation study. The best results appear in \bf{bold}. }
\label{append_epsilon}
\end{table*}
\begin{table*}[h]
\centering
\footnotesize
\resizebox{\linewidth}{!}{
% Please add the following required packages to your document preamble:
% \usepackage{multirow}
% Please add the following required packages to your document preamble:
% \usepackage{multirow}
\begin{tabular}{rr|rrrrr|rrrrr}
\hline
\multicolumn{1}{l}{} & \multicolumn{1}{l}{} & \multicolumn{5}{c}{\name}                                                   & \multicolumn{5}{c}{\name-no$M$}                                             \\
Instance             & BKS                  & Success        & Best(\%)                  & Average(\%)               & Trials & Time(s)  & Success        & Best(\%)                  & Average(\%)               & Trials & Time(s)  \\ \hline
a280                 & 2579                 & \textbf{10/10} & \textbf{2579(0.0000)}     & \textbf{2579(0.0000)}     & 2.4    & 0.025    & \textbf{10/10} & \textbf{2579(0.0000)}     & \textbf{2579(0.0000)}     & 2.4    & 0.02     \\
ali535               & 202339               & \textbf{10/10} & \textbf{202339(0.0000)}   & \textbf{202339(0.0000)}   & 4.2    & 0.325    & \textbf{10/10} & \textbf{202339(0.0000)}   & \textbf{202339(0.0000)}   & 6      & 0.226    \\
att532               & 27686                & \textbf{10/10} & \textbf{27686(0.0000)}    & \textbf{27686(0.0000)}    & 29.2   & 1.597    & \textbf{10/10} & \textbf{27686(0.0000)}    & \textbf{27686(0.0000)}    & 51.7   & 1.408    \\
bier127              & 118282               & \textbf{10/10} & \textbf{118282(0.0000)}   & \textbf{118282(0.0000)}   & 1.9    & 0.019    & \textbf{10/10} & \textbf{118282(0.0000)}   & \textbf{118282(0.0000)}   & 1.7    & 0.01     \\
brg180               & 1950                 & \textbf{10/10} & \textbf{1950(0.0000)}     & \textbf{1950(0.0000)}     & 3.9    & 0.006    & \textbf{10/10} & \textbf{1950(0.0000)}     & \textbf{1950(0.0000)}     & 6.1    & 0.006    \\
ch130                & 6110                 & \textbf{10/10} & \textbf{6110(0.0000)}     & \textbf{6110(0.0000)}     & 4      & 0.017    & \textbf{10/10} & \textbf{6110(0.0000)}     & \textbf{6110(0.0000)}     & 3.2    & 0.008    \\
ch150                & 6528                 & \textbf{10/10} & \textbf{6528(0.0000)}     & \textbf{6528(0.0000)}     & 27.3   & 0.056    & \textbf{10/10} & \textbf{6528(0.0000)}     & \textbf{6528(0.0000)}     & 31.5   & 0.082    \\
d1291                & 50801                & \textbf{10/10} & \textbf{50801(0.0000)}    & \textbf{50801(0.0000)}    & 170.1  & 16.348   & \textbf{10/10} & \textbf{50801(0.0000)}    & \textbf{50801(0.0000)}    & 169.4  & 9.709    \\
d1655                & 62128                & \textbf{10/10} & \textbf{62128(0.0000)}    & \textbf{62128(0.0000)}    & 39.3   & 1.108    & \textbf{10/10} & \textbf{62128(0.0000)}    & \textbf{62128(0.0000)}    & 27.8   & 0.845    \\
d198                 & 15780                & \textbf{10/10} & \textbf{15780(0.0000)}    & \textbf{15780(0.0000)}    & 18.3   & 0.454    & \textbf{10/10} & \textbf{15780(0.0000)}    & \textbf{15780(0.0000)}    & 12.8   & 0.234    \\
d2103                & 80450                & \textbf{6/10}  & \textbf{80450(0.0000)}    & \textbf{80451.5(0.0019)}  & 945.7  & 474.485  & \textbf{7/10}  & \textbf{80450(0.0000)}    & \textbf{80451.2(0.0015)}  & 1179.7 & 283.459  \\
d493                 & 35002                & \textbf{10/10} & \textbf{35002(0.0000)}    & \textbf{35002(0.0000)}    & 50.7   & 1.687    & \textbf{10/10} & \textbf{35002(0.0000)}    & \textbf{35002(0.0000)}    & 22.4   & 0.581    \\
d657                 & 48912                & \textbf{10/10} & \textbf{48912(0.0000)}    & \textbf{48912(0.0000)}    & 25.7   & 0.673    & \textbf{10/10} & \textbf{48912(0.0000)}    & \textbf{48912(0.0000)}    & 34.5   & 0.547    \\
dsj1000              & 18660188             & \textbf{10/10} & \textbf{18660188(0.0000)} & \textbf{18660188(0.0000)} & 31     & 9.069    & \textbf{10/10} & \textbf{18660188(0.0000)} & \textbf{18660188(0.0000)} & 51.6   & 8.316    \\
eil101               & 629                  & \textbf{10/10} & \textbf{629(0.0000)}      & \textbf{629(0.0000)}      & 1      & 0.005    & \textbf{10/10} & \textbf{629(0.0000)}      & \textbf{629(0.0000)}      & 1.1    & 0.006    \\
fl1400               & 20127                & \textbf{3/10}  & \textbf{20127(0.0000)}    & \textbf{20152.9(0.1287)}  & 1115.4 & 426.471  & 2/10           & \textbf{20127(0.0000)}    & 20156.7(0.1476)           & 1139.9 & 226.707  \\
fl1577               & 22249                & \textbf{10/10} & \textbf{22249(0.0000)}    & \textbf{22249(0.0000)}    & 303.5  & 3112.618 & \textbf{9/10}  & \textbf{22249(0.0000)}    & \textbf{22250.2(0.0054)}  & 354    & 966.433  \\
fl3795               & 28772                & \textbf{4/10}  & \textbf{28772(0.0000)}    & \textbf{28779.8(0.0271)}  & 2590.4 & 2379.836 & \textbf{5/10}  & \textbf{28772(0.0000)}    & \textbf{28781.3(0.0323)}  & 2809.2 & 1286.921 \\
fl417                & 11861                & \textbf{10/10} & \textbf{11861(0.0000)}    & \textbf{11861(0.0000)}    & 7.2    & 13.871   & \textbf{10/10} & \textbf{11861(0.0000)}    & \textbf{11861(0.0000)}    & 13.8   & 6.28     \\
fnl4461              & 182566               & \textbf{10/10} & \textbf{182566(0.0000)}   & \textbf{182566(0.0000)}   & 322.4  & 74.652   & \textbf{10/10} & \textbf{182566(0.0000)}   & \textbf{182566(0.0000)}   & 363.1  & 58.861   \\
gil262               & 2378                 & \textbf{10/10} & \textbf{2378(0.0000)}     & \textbf{2378(0.0000)}     & 7      & 0.247    & \textbf{10/10} & \textbf{2378(0.0000)}     & \textbf{2378(0.0000)}     & 14.6   & 0.177    \\
gr120                & 6942                 & \textbf{10/10} & \textbf{6942(0.0000)}     & \textbf{6942(0.0000)}     & 4.5    & 0.009    & \textbf{10/10} & \textbf{6942(0.0000)}     & \textbf{6942(0.0000)}     & 3.1    & 0.007    \\
gr137                & 69853                & 9/10           & \textbf{69853(0.0000)}    & 69865.7(0.0182)           & 14.6   & 0.024    & \textbf{10/10} & \textbf{69853(0.0000)}    & \textbf{69853(0.0000)}    & 10.3   & 0.011    \\
gr202                & 40160                & \textbf{10/10} & \textbf{40160(0.0000)}    & \textbf{40160(0.0000)}    & 2.4    & 0.029    & \textbf{10/10} & \textbf{40160(0.0000)}    & \textbf{40160(0.0000)}    & 12.4   & 0.016    \\
gr229                & 134602               & \textbf{10/10} & \textbf{134602(0.0000)}   & \textbf{134602(0.0000)}   & 22     & 0.096    & \textbf{10/10} & \textbf{134602(0.0000)}   & \textbf{134602(0.0000)}   & 11.9   & 0.07     \\
gr431                & 171414               & \textbf{10/10} & \textbf{171414(0.0000)}   & \textbf{171414(0.0000)}   & 107    & 2.997    & \textbf{10/10} & \textbf{171414(0.0000)}   & \textbf{171414(0.0000)}   & 98.7   & 2.869    \\
gr666                & 294358               & 7/10           & \textbf{294358(0.0000)}   & 294393.4(0.0120)          & 372.4  & 9.903    & \textbf{10/10} & \textbf{294358(0.0000)}   & \textbf{294358(0.0000)}   & 204.8  & 4.683    \\
kroA150              & 26524                & \textbf{10/10} & \textbf{26524(0.0000)}    & \textbf{26524(0.0000)}    & 2.3    & 0.074    & \textbf{10/10} & \textbf{26524(0.0000)}    & \textbf{26524(0.0000)}    & 6.6    & 0.034    \\
kroA200              & 29368                & \textbf{10/10} & \textbf{29368(0.0000)}    & \textbf{29368(0.0000)}    & 2.5    & 0.156    & \textbf{10/10} & \textbf{29368(0.0000)}    & \textbf{29368(0.0000)}    & 3.4    & 0.096    \\
kroB150              & 26130                & \textbf{8/10}  & \textbf{26130(0.0000)}    & \textbf{26130.4(0.0015)}  & 51.7   & 0.222    & 7/10           & \textbf{26130(0.0000)}    & 26130.6(0.0023)           & 68.8   & 0.168    \\
kroB200              & 29437                & \textbf{10/10} & \textbf{29437(0.0000)}    & \textbf{29437(0.0000)}    & 2.1    & 0.067    & \textbf{10/10} & \textbf{29437(0.0000)}    & \textbf{29437(0.0000)}    & 5      & 0.042    \\
lin105               & 14379                & \textbf{10/10} & \textbf{14379(0.0000)}    & \textbf{14379(0.0000)}    & 1      & 0.002    & \textbf{10/10} & \textbf{14379(0.0000)}    & \textbf{14379(0.0000)}    & 1      & 0.002    \\
lin318               & 42029                & \textbf{8/10}  & \textbf{42029(0.0000)}    & \textbf{42051.8(0.0542)}  & 140.8  & 0.525    & 5/10           & \textbf{42029(0.0000)}    & \textbf{42084.6(0.1323)}  & 241.5  & 0.655    \\
lin318               & 41345                & \textbf{10/10} & \textbf{41345(0.0000)}    & \textbf{41345(0.0000)}    & 16.7   & 0.087    & \textbf{10/10} & \textbf{41345(0.0000)}    & \textbf{41345(0.0000)}    & 9.5    & 0.058    \\
nrw1379              & 56638                & \textbf{10/10} & \textbf{56638(0.0000)}    & \textbf{56638(0.0000)}    & 476.9  & 23.146   & 9/10           & \textbf{56638(0.0000)}    & \textbf{56638.5(0.0009)}  & 391.6  & 12.211   \\
p654                 & 34643                & \textbf{10/10} & \textbf{34643(0.0000)}    & \textbf{34643(0.0000)}    & 15.6   & 45.578   & \textbf{10/10} & \textbf{34643(0.0000)}    & \textbf{34643(0.0000)}    & 19.1   & 6.946    \\
pa561.tsp            & 2763                 & \textbf{10/10} & \textbf{2763(0.0000)}     & \textbf{2763(0.0000)}     & 13.7   & 0.81     & \textbf{10/10} & \textbf{2763(0.0000)}     & \textbf{2763(0.0000)}     & 13.7   & 0.326    \\
pcb1173              & 56892                & \textbf{6/10}  & \textbf{56892(0.0000)}    & \textbf{56894(0.0035)}    & 721.2  & 15.051   & \textbf{6/10}  & \textbf{56892(0.0000)}    & \textbf{56894(0.0035)}    & 696.9  & 11.571   \\
pcb3038              & 137694               & \textbf{9/10}  & \textbf{137694(0.0000)}   & \textbf{137694.5(0.0004)} & 1021.9 & 167.493  & \textbf{8/10}  & \textbf{137694(0.0000)}   & \textbf{137699.2(0.0038)} & 963.8  & 103.78   \\
pcb442               & 50778                & \textbf{10/10} & \textbf{50778(0.0000)}    & \textbf{50778(0.0000)}    & 4.8    & 0.185    & \textbf{10/10} & \textbf{50778(0.0000)}    & \textbf{50778(0.0000)}    & 12.5   & 0.196    \\
pla7397              & 23260728             & \textbf{10/10} & \textbf{23260728(0.0000)} & \textbf{23260728(0.0000)} & 206.4  & 889.849  & \textbf{10/10} & \textbf{23260728(0.0000)} & \textbf{23260728(0.0000)} & 1124   & 1375.695 \\
pr1002               & 259045               & \textbf{10/10} & \textbf{259045(0.0000)}   & \textbf{259045(0.0000)}   & 281.1  & 4.893    & \textbf{10/10} & \textbf{259045(0.0000)}   & \textbf{259045(0.0000)}   & 57     & 1.563    \\
pr107                & 44303                & \textbf{10/10} & \textbf{44303(0.0000)}    & \textbf{44303(0.0000)}    & 1.7    & 0.106    & \textbf{10/10} & \textbf{44303(0.0000)}    & \textbf{44303(0.0000)}    & 1      & 0.076    \\
pr124                & 59030                & \textbf{10/10} & \textbf{59030(0.0000)}    & \textbf{59030(0.0000)}    & 2.2    & 0.03     & \textbf{10/10} & \textbf{59030(0.0000)}    & \textbf{59030(0.0000)}    & 2      & 0.03     \\
pr136                & 96772                & \textbf{10/10} & \textbf{96772(0.0000)}    & \textbf{96772(0.0000)}    & 1.8    & 0.314    & \textbf{10/10} & \textbf{96772(0.0000)}    & \textbf{96772(0.0000)}    & 4.4    & 0.146    \\
pr144                & 58537                & \textbf{10/10} & \textbf{58537(0.0000)}    & \textbf{58537(0.0000)}    & 2.9    & 0.98     & \textbf{10/10} & \textbf{58537(0.0000)}    & \textbf{58537(0.0000)}    & 3.8    & 1.049    \\
pr152                & 73682                & \textbf{10/10} & \textbf{73682(0.0000)}    & \textbf{73682(0.0000)}    & 9.7    & 3.531    & \textbf{10/10} & \textbf{73682(0.0000)}    & \textbf{73682(0.0000)}    & 22.5   & 0.614    \\
pr226                & 80369                & \textbf{10/10} & \textbf{80369(0.0000)}    & \textbf{80369(0.0000)}    & 12.4   & 0.591    & \textbf{10/10} & \textbf{80369(0.0000)}    & \textbf{80369(0.0000)}    & 9.1    & 0.121    \\
pr2392               & 378032               & \textbf{10/10} & \textbf{378032(0.0000)}   & \textbf{378032(0.0000)}   & 13.3   & 42.932   & \textbf{10/10} & \textbf{378032(0.0000)}   & \textbf{378032(0.0000)}   & 23.4   & 30.742   \\
pr299                & 48191                & \textbf{10/10} & \textbf{48191(0.0000)}    & \textbf{48191(0.0000)}    & 3.3    & 0.488    & \textbf{10/10} & \textbf{48191(0.0000)}    & \textbf{48191(0.0000)}    & 7.6    & 0.299    \\
pr439                & 107217               & \textbf{10/10} & \textbf{107217(0.0000)}   & \textbf{107217(0.0000)}   & 65.1   & 1.86     & \textbf{10/10} & \textbf{107217(0.0000)}   & \textbf{107217(0.0000)}   & 59.5   & 1.015    \\
rat195               & 2323                 & \textbf{10/10} & \textbf{2323(0.0000)}     & \textbf{2323(0.0000)}     & 24.7   & 0.285    & \textbf{10/10} & \textbf{2323(0.0000)}     & \textbf{2323(0.0000)}     & 5.2    & 0.12     \\
rat575               & 6773                 & \textbf{7/10}  & \textbf{6773(0.0000)}     & \textbf{6773.4(0.0059)}   & 286.9  & 3.388    & 5/10           & \textbf{6773(0.0000)}     & 6773.5(0.0074)            & 411.6  & 4.293    \\
rat783               & 8806                 & \textbf{10/10} & \textbf{8806(0.0000)}     & \textbf{8806(0.0000)}     & 18.4   & 0.595    & \textbf{10/10} & \textbf{8806(0.0000)}     & \textbf{8806(0.0000)}     & 31.5   & 0.411    \\
rd400                & 15281                & \textbf{10/10} & \textbf{15281(0.0000)}    & \textbf{15281(0.0000)}    & 34     & 0.534    & \textbf{10/10} & \textbf{15281(0.0000)}    & \textbf{15281(0.0000)}    & 8.8    & 0.206    \\
rl1304               & 252948               & \textbf{8/10}  & \textbf{252948(0.0000)}   & 252991.3(0.0171)          & 493.4  & 19.742   & \textbf{10/10} & \textbf{252948(0.0000)}   & \textbf{252948(0.0000)}   & 325.6  & 9.521    \\
rl1323               & 270199               & \textbf{9/10}  & \textbf{270199(0.0000)}   & \textbf{270201.7(0.0010)} & 358.2  & 18.002   & \textbf{9/10}  & \textbf{270199(0.0000)}   & \textbf{270201.7(0.0010)} & 283    & 8.996    \\
rl1889               & 316536               & \textbf{10/10} & \textbf{316536(0.0000)}   & \textbf{316536(0.0000)}   & 420.2  & 91.595   & 8/10           & \textbf{316536(0.0000)}   & 316558.8(0.0072)          & 821.4  & 75.317   \\
rl5915               & 565530               & \textbf{2/10}  & \textbf{565530(0.0000)}   & \textbf{565573.3(0.0077)} & 4927.6 & 1521.327 & \textbf{1/10}  & \textbf{565530(0.0000)}   & \textbf{565577.4(0.0084)} & 5399.4 & 1288.736 \\
rl5934               & 556045               & \textbf{5/10}  & \textbf{556045(0.0000)}   & \textbf{556130.2(0.0153)} & 4207.3 & 2004.291 & \textbf{8/10}  & \textbf{556045(0.0000)}   & \textbf{556063.2(0.0033)} & 3445.9 & 1426.989 \\
si1032               & 92650                & \textbf{10/10} & \textbf{92650(0.0000)}    & \textbf{92650(0.0000)}    & 15.5   & 87.295   & \textbf{10/10} & \textbf{92650(0.0000)}    & \textbf{92650(0.0000)}    & 19.8   & 17.698   \\
si175                & 21407                & 7/10           & \textbf{21407(0.0000)}    & 21407.3(0.0014)           & 69.2   & 8.273    & \textbf{10/10} & \textbf{21407(0.0000)}    & \textbf{21407(0.0000)}    & 34.6   & 3.126    \\
si535                & 48450                & \textbf{8/10}  & \textbf{48450(0.0000)}    & \textbf{48450.6(0.0012)}  & 192.8  & 77.812   & \textbf{10/10} & \textbf{48450(0.0000)}    & \textbf{48450(0.0000)}    & 94.4   & 14.403   \\
ts225                & 126643               & \textbf{10/10} & \textbf{126643(0.0000)}   & \textbf{126643(0.0000)}   & 1      & 0.027    & \textbf{10/10} & \textbf{126643(0.0000)}   & \textbf{126643(0.0000)}   & 1      & 0.026    \\
tsp225               & 3916                 & \textbf{10/10} & \textbf{3916(0.0000)}     & \textbf{3916(0.0000)}     & 3.5    & 0.132    & \textbf{10/10} & \textbf{3916(0.0000)}     & \textbf{3916(0.0000)}     & 4      & 0.044    \\
u1060                & 224094               & \textbf{10/10} & \textbf{224094(0.0000)}   & \textbf{224094(0.0000)}   & 113.1  & 113.18   & \textbf{10/10} & \textbf{224094(0.0000)}   & \textbf{224094(0.0000)}   & 18.4   & 5.216    \\
u1432                & 152970               & \textbf{10/10} & \textbf{152970(0.0000)}   & \textbf{152970(0.0000)}   & 9.5    & 1.325    & \textbf{10/10} & \textbf{152970(0.0000)}   & \textbf{152970(0.0000)}   & 13.4   & 0.956    \\
u159                 & 42080                & \textbf{10/10} & \textbf{42080(0.0000)}    & \textbf{42080(0.0000)}    & 2.8    & 0.017    & \textbf{10/10} & \textbf{42080(0.0000)}    & \textbf{42080(0.0000)}    & 2      & 0.017    \\
u1817                & 57201                & \textbf{0/10}  & \textbf{57216(0.0262)}    & \textbf{57242.3(0.0722)}  & 1817   & 481.484  & \textbf{0/10}  & \textbf{57225(0.0420)}    & \textbf{57242.3(0.0722)}  & 1817   & 244.458  \\
u2152                & 64253                & \textbf{9/10}  & \textbf{64253(0.0000)}    & \textbf{64257(0.0062)}    & 800.9  & 160.547  & \textbf{8/10}  & \textbf{64253(0.0000)}    & \textbf{64259.8(0.0106)}  & 844    & 99.623   \\
u2319                & 234256               & \textbf{10/10} & \textbf{234256(0.0000)}   & \textbf{234256(0.0000)}   & 17.8   & 6.453    & \textbf{10/10} & \textbf{234256(0.0000)}   & \textbf{234256(0.0000)}   & 15     & 2.379    \\
u574                 & 36905                & \textbf{10/10} & \textbf{36905(0.0000)}    & \textbf{36905(0.0000)}    & 33     & 1.126    & \textbf{10/10} & \textbf{36905(0.0000)}    & \textbf{36905(0.0000)}    & 16.9   & 0.404    \\
u724                 & 41910                & \textbf{10/10} & \textbf{41910(0.0000)}    & \textbf{41910(0.0000)}    & 90.6   & 3.3      & \textbf{10/10} & \textbf{41910(0.0000)}    & \textbf{41910(0.0000)}    & 97.7   & 2.918    \\
vm1084               & 239297               & \textbf{8/10}  & \textbf{239297(0.0000)}   & \textbf{239307.4(0.0043)} & 419.8  & 51.722   & \textbf{10/10} & \textbf{239297(0.0000)}   & \textbf{239297(0.0000)}   & 99.2   & 6.392    \\
vm1748               & 336556               & \textbf{10/10} & \textbf{336556(0.0000)}   & \textbf{336556(0.0000)}   & 257.7  & 18.207   & \textbf{9/10}  & \textbf{336556(0.0000)}   & \textbf{336570.5(0.0043)} & 702.8  & 29.645   \\ \hline
                     & Average Gap(\%)      &                & \textbf{0.0003}           & \textbf{0.0051}           &        &          &                & 0.0059                    & 0.0139                    &        &     \\ \hline    
\end{tabular}
}
\caption{Full comparisonal results of \name and \name-no$M$ in ablation study. The best results appear in \bf{bold}. }
\label{appendix_M}
\end{table*}
\begin{table*}[h]
\centering
\footnotesize
\resizebox{\linewidth}{!}{
% Please add the following required packages to your document preamble:
% \usepackage{multirow}
\begin{tabular}{rr|rrrrr|rrrrr}
\hline
\multicolumn{1}{l}{} & \multicolumn{1}{l}{} & \multicolumn{5}{c}{\name}                                                   & \multicolumn{5}{c}{\name-no$\alpha$}                                        \\
Instance             & BKS                  & Success        & Best(\%)                  & Average(\%)               & Trials & Time(s)  & Success        & Best(\%)                  & Average(\%)               & Trials & Time(s)  \\ \hline
a280                 & 2579                 & \textbf{10/10} & \textbf{2579(0.0000)}     & \textbf{2579(0.0000)}     & 2.4    & 0.025    & \textbf{10/10} & \textbf{2579(0.0000)}     & \textbf{2579(0.0000)}     & 2.4    & 0.02     \\
ali535               & 202339               & \textbf{10/10} & \textbf{202339(0.0000)}   & \textbf{202339(0.0000)}   & 4.2    & 0.325    & \textbf{10/10} & \textbf{202339(0.0000)}   & \textbf{202339(0.0000)}   & 6      & 0.23     \\
att532               & 27686                & \textbf{10/10} & \textbf{27686(0.0000)}    & \textbf{27686(0.0000)}    & 29.2   & 1.597    & \textbf{10/10} & \textbf{27686(0.0000)}    & \textbf{27686(0.0000)}    & 66.8   & 1.698    \\
bier127              & 118282               & \textbf{10/10} & \textbf{118282(0.0000)}   & \textbf{118282(0.0000)}   & 1.9    & 0.019    & \textbf{10/10} & \textbf{118282(0.0000)}   & \textbf{118282(0.0000)}   & 1.7    & 0.01     \\
brg180               & 1950                 & \textbf{10/10} & \textbf{1950(0.0000)}     & \textbf{1950(0.0000)}     & 3.9    & 0.006    & \textbf{10/10} & \textbf{1950(0.0000)}     & \textbf{1950(0.0000)}     & 6.1    & 0.005    \\
ch130                & 6110                 & \textbf{10/10} & \textbf{6110(0.0000)}     & \textbf{6110(0.0000)}     & 4      & 0.017    & \textbf{10/10} & \textbf{6110(0.0000)}     & \textbf{6110(0.0000)}     & 3.3    & 0.013    \\
ch150                & 6528                 & \textbf{10/10} & \textbf{6528(0.0000)}     & \textbf{6528(0.0000)}     & 27.3   & 0.056    & \textbf{10/10} & \textbf{6528(0.0000)}     & \textbf{6528(0.0000)}     & 33.5   & 0.076    \\
d1291                & 50801                & \textbf{10/10} & \textbf{50801(0.0000)}    & \textbf{50801(0.0000)}    & 170.1  & 16.348   & \textbf{10/10} & \textbf{50801(0.0000)}    & \textbf{50801(0.0000)}    & 230.6  & 11.894   \\
d1655                & 62128                & \textbf{10/10} & \textbf{62128(0.0000)}    & \textbf{62128(0.0000)}    & 39.3   & 1.108    & \textbf{10/10} & \textbf{62128(0.0000)}    & \textbf{62128(0.0000)}    & 37.4   & 1.096    \\
d198                 & 15780                & \textbf{10/10} & \textbf{15780(0.0000)}    & \textbf{15780(0.0000)}    & 18.3   & 0.454    & \textbf{10/10} & \textbf{15780(0.0000)}    & \textbf{15780(0.0000)}    & 12.8   & 0.233    \\
d2103                & 80450                & \textbf{6/10}  & \textbf{80450(0.0000)}    & \textbf{80451.5(0.0019)}  & 945.7  & 474.485  & \textbf{5/10}  & \textbf{80450(0.0000)}    & \textbf{80451.6(0.0020)}  & 1351.8 & 267.869  \\
d493                 & 35002                & \textbf{10/10} & \textbf{35002(0.0000)}    & \textbf{35002(0.0000)}    & 50.7   & 1.687    & \textbf{10/10} & \textbf{35002(0.0000)}    & \textbf{35002(0.0000)}    & 30.2   & 0.813    \\
d657                 & 48912                & \textbf{10/10} & \textbf{48912(0.0000)}    & \textbf{48912(0.0000)}    & 25.7   & 0.673    & \textbf{10/10} & \textbf{48912(0.0000)}    & \textbf{48912(0.0000)}    & 23.5   & 0.359    \\
dsj1000              & 18660188             & \textbf{10/10} & \textbf{18660188(0.0000)} & \textbf{18660188(0.0000)} & 31     & 9.069    & \textbf{10/10} & \textbf{18660188(0.0000)} & \textbf{18660188(0.0000)} & 51.6   & 8.318    \\
eil101               & 629                  & \textbf{10/10} & \textbf{629(0.0000)}      & \textbf{629(0.0000)}      & 1      & 0.005    & \textbf{10/10} & \textbf{629(0.0000)}      & \textbf{629(0.0000)}      & 2.5    & 0.006    \\
fl1400               & 20127                & \textbf{3/10}  & \textbf{20127(0.0000)}    & \textbf{20152.9(0.1287)}  & 1115.4 & 426.471  & 2/10           & \textbf{20127(0.0000)}    & 20156.6(0.1471)           & 1127   & 231.962  \\
fl1577               & 22249                & \textbf{10/10} & \textbf{22249(0.0000)}    & \textbf{22249(0.0000)}    & 303.5  & 3112.618 & \textbf{10/10} & \textbf{22249(0.0000)}    & \textbf{22249(0.0000)}    & 378.2  & 1180.205 \\
fl3795               & 28772                & \textbf{4/10}  & \textbf{28772(0.0000)}    & \textbf{28779.8(0.0271)}  & 2590.4 & 2379.836 & \textbf{2/10}  & \textbf{28772(0.0000)}    & \textbf{28788(0.0556)}    & 3067.3 & 1422.153 \\
fl417                & 11861                & \textbf{10/10} & \textbf{11861(0.0000)}    & \textbf{11861(0.0000)}    & 7.2    & 13.871   & \textbf{10/10} & \textbf{11861(0.0000)}    & \textbf{11861(0.0000)}    & 30.6   & 11.105   \\
fnl4461              & 182566               & \textbf{10/10} & \textbf{182566(0.0000)}   & \textbf{182566(0.0000)}   & 322.4  & 74.652   & \textbf{10/10} & \textbf{182566(0.0000)}   & \textbf{182566(0.0000)}   & 740.9  & 86.895   \\
gil262               & 2378                 & \textbf{10/10} & \textbf{2378(0.0000)}     & \textbf{2378(0.0000)}     & 7      & 0.247    & \textbf{10/10} & \textbf{2378(0.0000)}     & \textbf{2378(0.0000)}     & 13.1   & 0.151    \\
gr120                & 6942                 & \textbf{10/10} & \textbf{6942(0.0000)}     & \textbf{6942(0.0000)}     & 4.5    & 0.009    & \textbf{10/10} & \textbf{6942(0.0000)}     & \textbf{6942(0.0000)}     & 3.1    & 0.007    \\
gr137                & 69853                & 9/10           & \textbf{69853(0.0000)}    & 69865.7(0.0182)           & 14.6   & 0.024    & \textbf{10/10} & \textbf{69853(0.0000)}    & \textbf{69853(0.0000)}    & 10.3   & 0.011    \\
gr202                & 40160                & \textbf{10/10} & \textbf{40160(0.0000)}    & \textbf{40160(0.0000)}    & 2.4    & 0.029    & \textbf{9/10}  & \textbf{40160(0.0000)}    & \textbf{40160.1(0.0002)}  & 41     & 0.025    \\
gr229                & 134602               & \textbf{10/10} & \textbf{134602(0.0000)}   & \textbf{134602(0.0000)}   & 22     & 0.096    & \textbf{10/10} & \textbf{134602(0.0000)}   & \textbf{134602(0.0000)}   & 11.9   & 0.07     \\
gr431                & 171414               & \textbf{10/10} & \textbf{171414(0.0000)}   & \textbf{171414(0.0000)}   & 107    & 2.997    & \textbf{10/10} & \textbf{171414(0.0000)}   & \textbf{171414(0.0000)}   & 89.8   & 2.387    \\
gr666                & 294358               & 7/10           & \textbf{294358(0.0000)}   & 294393.4(0.0120)          & 372.4  & 9.903    & \textbf{8/10}  & \textbf{294358(0.0000)}   & \textbf{294381.8(0.0081)} & 281.1  & 6.029    \\
kroA150              & 26524                & \textbf{10/10} & \textbf{26524(0.0000)}    & \textbf{26524(0.0000)}    & 2.3    & 0.074    & \textbf{10/10} & \textbf{26524(0.0000)}    & \textbf{26524(0.0000)}    & 3.1    & 0.041    \\
kroA200              & 29368                & \textbf{10/10} & \textbf{29368(0.0000)}    & \textbf{29368(0.0000)}    & 2.5    & 0.156    & \textbf{10/10} & \textbf{29368(0.0000)}    & \textbf{29368(0.0000)}    & 5.2    & 0.11     \\
kroB150              & 26130                & \textbf{8/10}  & \textbf{26130(0.0000)}    & \textbf{26130.4(0.0015)}  & 51.7   & 0.222    & 4/10           & \textbf{26130(0.0000)}    & 26131.2(0.0046)           & 106    & 0.288    \\
kroB200              & 29437                & \textbf{10/10} & \textbf{29437(0.0000)}    & \textbf{29437(0.0000)}    & 2.1    & 0.067    & \textbf{10/10} & \textbf{29437(0.0000)}    & \textbf{29437(0.0000)}    & 23.6   & 0.07     \\
lin105               & 14379                & \textbf{10/10} & \textbf{14379(0.0000)}    & \textbf{14379(0.0000)}    & 1      & 0.002    & \textbf{10/10} & \textbf{14379(0.0000)}    & \textbf{14379(0.0000)}    & 1      & 0.002    \\
lin318               & 42029                & \textbf{8/10}  & \textbf{42029(0.0000)}    & \textbf{42051.8(0.0542)}  & 140.8  & 0.525    & 4/10           & \textbf{42029(0.0000)}    & \textbf{42096(0.1594)}    & 233.1  & 0.558    \\
lin318               & 41345                & \textbf{10/10} & \textbf{41345(0.0000)}    & \textbf{41345(0.0000)}    & 16.7   & 0.087    & \textbf{10/10} & \textbf{41345(0.0000)}    & \textbf{41345(0.0000)}    & 15     & 0.055    \\
nrw1379              & 56638                & \textbf{10/10} & \textbf{56638(0.0000)}    & \textbf{56638(0.0000)}    & 476.9  & 23.146   & 8/10           & \textbf{56638(0.0000)}    & \textbf{56639(0.0018)}    & 426.9  & 12.296   \\
p654                 & 34643                & \textbf{10/10} & \textbf{34643(0.0000)}    & \textbf{34643(0.0000)}    & 15.6   & 45.578   & \textbf{10/10} & \textbf{34643(0.0000)}    & \textbf{34643(0.0000)}    & 12.7   & 6.092    \\
pa561.tsp            & 2763                 & \textbf{10/10} & \textbf{2763(0.0000)}     & \textbf{2763(0.0000)}     & 13.7   & 0.81     & \textbf{10/10} & \textbf{2763(0.0000)}     & \textbf{2763(0.0000)}     & 20.9   & 0.667    \\
pcb1173              & 56892                & \textbf{6/10}  & \textbf{56892(0.0000)}    & \textbf{56894(0.0035)}    & 721.2  & 15.051   & \textbf{7/10}  & \textbf{56892(0.0000)}    & \textbf{56893.5(0.0026)}  & 590.8  & 10.679   \\
pcb3038              & 137694               & \textbf{9/10}  & \textbf{137694(0.0000)}   & \textbf{137694.5(0.0004)} & 1021.9 & 167.493  & \textbf{9/10}  & \textbf{137694(0.0000)}   & \textbf{137694.5(0.0004)} & 562.9  & 68.348   \\
pcb442               & 50778                & \textbf{10/10} & \textbf{50778(0.0000)}    & \textbf{50778(0.0000)}    & 4.8    & 0.185    & \textbf{10/10} & \textbf{50778(0.0000)}    & \textbf{50778(0.0000)}    & 7.3    & 0.14     \\
pla7397              & 23260728             & \textbf{10/10} & \textbf{23260728(0.0000)} & \textbf{23260728(0.0000)} & 206.4  & 889.849  & \textbf{10/10} & \textbf{23260728(0.0000)} & \textbf{23260728(0.0000)} & 720.6  & 769.684  \\
pr1002               & 259045               & \textbf{10/10} & \textbf{259045(0.0000)}   & \textbf{259045(0.0000)}   & 281.1  & 4.893    & \textbf{10/10} & \textbf{259045(0.0000)}   & \textbf{259045(0.0000)}   & 263.9  & 3.443    \\
pr107                & 44303                & \textbf{10/10} & \textbf{44303(0.0000)}    & \textbf{44303(0.0000)}    & 1.7    & 0.106    & \textbf{10/10} & \textbf{44303(0.0000)}    & \textbf{44303(0.0000)}    & 1      & 0.125    \\
pr124                & 59030                & \textbf{10/10} & \textbf{59030(0.0000)}    & \textbf{59030(0.0000)}    & 2.2    & 0.03     & \textbf{10/10} & \textbf{59030(0.0000)}    & \textbf{59030(0.0000)}    & 1.7    & 0.087    \\
pr136                & 96772                & \textbf{10/10} & \textbf{96772(0.0000)}    & \textbf{96772(0.0000)}    & 1.8    & 0.314    & \textbf{10/10} & \textbf{96772(0.0000)}    & \textbf{96772(0.0000)}    & 1.9    & 0.104    \\
pr144                & 58537                & \textbf{10/10} & \textbf{58537(0.0000)}    & \textbf{58537(0.0000)}    & 2.9    & 0.98     & \textbf{10/10} & \textbf{58537(0.0000)}    & \textbf{58537(0.0000)}    & 2      & 1.255    \\
pr152                & 73682                & \textbf{10/10} & \textbf{73682(0.0000)}    & \textbf{73682(0.0000)}    & 9.7    & 3.531    & \textbf{10/10} & \textbf{73682(0.0000)}    & \textbf{73682(0.0000)}    & 38.6   & 0.96     \\
pr226                & 80369                & \textbf{10/10} & \textbf{80369(0.0000)}    & \textbf{80369(0.0000)}    & 12.4   & 0.591    & \textbf{10/10} & \textbf{80369(0.0000)}    & \textbf{80369(0.0000)}    & 16.8   & 0.163    \\
pr2392               & 378032               & \textbf{10/10} & \textbf{378032(0.0000)}   & \textbf{378032(0.0000)}   & 13.3   & 42.932   & \textbf{10/10} & \textbf{378032(0.0000)}   & \textbf{378032(0.0000)}   & 24.2   & 29.319   \\
pr299                & 48191                & \textbf{10/10} & \textbf{48191(0.0000)}    & \textbf{48191(0.0000)}    & 3.3    & 0.488    & \textbf{10/10} & \textbf{48191(0.0000)}    & \textbf{48191(0.0000)}    & 4.8    & 0.22     \\
pr439                & 107217               & \textbf{10/10} & \textbf{107217(0.0000)}   & \textbf{107217(0.0000)}   & 65.1   & 1.86     & \textbf{10/10} & \textbf{107217(0.0000)}   & \textbf{107217(0.0000)}   & 46.6   & 0.676    \\
rat195               & 2323                 & \textbf{10/10} & \textbf{2323(0.0000)}     & \textbf{2323(0.0000)}     & 24.7   & 0.285    & \textbf{9/10}  & \textbf{2323(0.0000)}     & \textbf{2323.5(0.0215)}   & 23.3   & 0.162    \\
rat575               & 6773                 & \textbf{7/10}  & \textbf{6773(0.0000)}     & \textbf{6773.4(0.0059)}   & 286.9  & 3.388    & 4/10           & \textbf{6773(0.0000)}     & 6773.6(0.0089)            & 412.6  & 3.785    \\
rat783               & 8806                 & \textbf{10/10} & \textbf{8806(0.0000)}     & \textbf{8806(0.0000)}     & 18.4   & 0.595    & \textbf{10/10} & \textbf{8806(0.0000)}     & \textbf{8806(0.0000)}     & 19.6   & 0.332    \\
rd400                & 15281                & \textbf{10/10} & \textbf{15281(0.0000)}    & \textbf{15281(0.0000)}    & 34     & 0.534    & \textbf{10/10} & \textbf{15281(0.0000)}    & \textbf{15281(0.0000)}    & 25.8   & 0.281    \\
rl1304               & 252948               & \textbf{8/10}  & \textbf{252948(0.0000)}   & 252991.3(0.0171)          & 493.4  & 19.742   & \textbf{8/10}  & \textbf{252948(0.0000)}   & \textbf{252987.9(0.0158)} & 486.6  & 12.321   \\
rl1323               & 270199               & \textbf{9/10}  & \textbf{270199(0.0000)}   & \textbf{270201.7(0.0010)} & 358.2  & 18.002   & \textbf{10/10} & \textbf{270199(0.0000)}   & \textbf{270199(0.0000)}   & 97.7   & 2.839    \\
rl1889               & 316536               & \textbf{10/10} & \textbf{316536(0.0000)}   & \textbf{316536(0.0000)}   & 420.2  & 91.595   & 9/10           & \textbf{316536(0.0000)}   & 316537.3(0.0004)          & 619.4  & 46.925   \\
rl5915               & 565530               & \textbf{2/10}  & \textbf{565530(0.0000)}   & \textbf{565573.3(0.0077)} & 4927.6 & 1521.327 & \textbf{2/10}  & \textbf{565530(0.0000)}   & \textbf{565571.9(0.0074)} & 5336.8 & 1312.179 \\
rl5934               & 556045               & \textbf{5/10}  & \textbf{556045(0.0000)}   & \textbf{556130.2(0.0153)} & 4207.3 & 2004.291 & \textbf{8/10}  & \textbf{556045(0.0000)}   & \textbf{556063.2(0.0033)} & 2739.9 & 1028.799 \\
si1032               & 92650                & \textbf{10/10} & \textbf{92650(0.0000)}    & \textbf{92650(0.0000)}    & 15.5   & 87.295   & \textbf{10/10} & \textbf{92650(0.0000)}    & \textbf{92650(0.0000)}    & 33.9   & 20.039   \\
si175                & 21407                & 7/10           & \textbf{21407(0.0000)}    & 21407.3(0.0014)           & 69.2   & 8.273    & \textbf{10/10} & \textbf{21407(0.0000)}    & \textbf{21407(0.0000)}    & 39.6   & 3.883    \\
si535                & 48450                & \textbf{8/10}  & \textbf{48450(0.0000)}    & \textbf{48450.6(0.0012)}  & 192.8  & 77.812   & \textbf{7/10}  & \textbf{48450(0.0000)}    & \textbf{48450.9(0.0019)}  & 188.9  & 27.383   \\
ts225                & 126643               & \textbf{10/10} & \textbf{126643(0.0000)}   & \textbf{126643(0.0000)}   & 1      & 0.027    & \textbf{10/10} & \textbf{126643(0.0000)}   & \textbf{126643(0.0000)}   & 1      & 0.028    \\
tsp225               & 3916                 & \textbf{10/10} & \textbf{3916(0.0000)}     & \textbf{3916(0.0000)}     & 3.5    & 0.132    & \textbf{10/10} & \textbf{3916(0.0000)}     & \textbf{3916(0.0000)}     & 2.8    & 0.029    \\
u1060                & 224094               & \textbf{10/10} & \textbf{224094(0.0000)}   & \textbf{224094(0.0000)}   & 113.1  & 113.18   & \textbf{10/10} & \textbf{224094(0.0000)}   & \textbf{224094(0.0000)}   & 30.4   & 8.385    \\
u1432                & 152970               & \textbf{10/10} & \textbf{152970(0.0000)}   & \textbf{152970(0.0000)}   & 9.5    & 1.325    & \textbf{10/10} & \textbf{152970(0.0000)}   & \textbf{152970(0.0000)}   & 16.6   & 1.587    \\
u159                 & 42080                & \textbf{10/10} & \textbf{42080(0.0000)}    & \textbf{42080(0.0000)}    & 2.8    & 0.017    & \textbf{10/10} & \textbf{42080(0.0000)}    & \textbf{42080(0.0000)}    & 1.8    & 0.014    \\
u1817                & 57201                & \textbf{0/10}  & \textbf{57216(0.0262)}    & \textbf{57242.3(0.0722)}  & 1817   & 481.484  & \textbf{0/10}  & \textbf{57238(0.0647)}    & \textbf{57246.6(0.0797)}  & 1817   & 222.875  \\
u2152                & 64253                & \textbf{9/10}  & \textbf{64253(0.0000)}    & \textbf{64257(0.0062)}    & 800.9  & 160.547  & \textbf{9/10}  & \textbf{64253(0.0000)}    & \textbf{64257(0.0062)}    & 818.1  & 85.978   \\
u2319                & 234256               & \textbf{10/10} & \textbf{234256(0.0000)}   & \textbf{234256(0.0000)}   & 17.8   & 6.453    & \textbf{10/10} & \textbf{234256(0.0000)}   & \textbf{234256(0.0000)}   & 14.7   & 2.325    \\
u574                 & 36905                & \textbf{10/10} & \textbf{36905(0.0000)}    & \textbf{36905(0.0000)}    & 33     & 1.126    & \textbf{10/10} & \textbf{36905(0.0000)}    & \textbf{36905(0.0000)}    & 7      & 0.263    \\
u724                 & 41910                & \textbf{10/10} & \textbf{41910(0.0000)}    & \textbf{41910(0.0000)}    & 90.6   & 3.3      & \textbf{10/10} & \textbf{41910(0.0000)}    & \textbf{41910(0.0000)}    & 92.1   & 2.842    \\
vm1084               & 239297               & \textbf{8/10}  & \textbf{239297(0.0000)}   & \textbf{239307.4(0.0043)} & 419.8  & 51.722   & \textbf{10/10} & \textbf{239297(0.0000)}   & \textbf{239297(0.0000)}   & 76.6   & 6.198    \\
vm1748               & 336556               & \textbf{10/10} & \textbf{336556(0.0000)}   & \textbf{336556(0.0000)}   & 257.7  & 18.207   & \textbf{10/10} & \textbf{336556(0.0000)}   & \textbf{336556(0.0000)}   & 537.5  & 27.089   \\ \hline
                     & Average Gap(\%)      &                & \textbf{0.0003}           & \textbf{0.0051}           &        &          &                & 0.0009                    & 0.0070                    &        &         \\ \hline
\end{tabular}
}
\caption{Full comparisonal results of \name and \name-no$\alpha$ in ablation study. The best results appear in \bf{bold}. }
\label{appendix_alpha}
\end{table*}

As shown in the three tables, no matter which method is missing, the experimental effect will decrease, that indicates the three strategy's cooperation is the most effective for algorithms to jump out of local optima.

\subsubsection{Full Results of Ablation Study on the MAB Model}
We set arms $m$ in MAB model is 4 in \ref{main_exep} with bigger candidate sets $C_{max}$, which equals to 7. In order to eliminate the impact of these two parameters on the experiment, We respectively conducted two ablation studies, setting the default number of candidate sets $k$ in LKH to 4 and 7, and compared them with the parameter $m$ set to 4, with $C_{max}$ set to 7 in \name.

\begin{table*}[h]
\centering
\footnotesize
\resizebox{\linewidth}{!}{
\begin{tabular}{rr|rrrrr|rrrrr}
\hline
\multicolumn{1}{l}{} & \multicolumn{1}{l}{} & \multicolumn{5}{c}{\name}                                                   & \multicolumn{5}{c}{\name-$m$}                                                \\
Instance             & BKS                  & Success        & Best(\%)                  & Average(\%)               & Trials & Time(s)  & Success        & Best(\%)                  & Average(\%)                 & Trials & Time(s) \\ \hline
a280                 & 2579                 & \textbf{10/10} & \textbf{2579(0.0000)}     & \textbf{2579(0.0000)}     & 2.4    & 0.025    & \textbf{10/10} & \textbf{2579(0.0000)}     & \textbf{2579(0.0000)}       & 1      & 0.01    \\
ali535               & 202339               & \textbf{10/10} & \textbf{202339(0.0000)}   & \textbf{202339(0.0000)}   & 4.2    & 0.325    & \textbf{6/10}  & \textbf{202339(0.0000)}   & \textbf{202355(0.0079)}     & 277    & 0.548   \\
att532               & 27686                & \textbf{10/10} & \textbf{27686(0.0000)}    & \textbf{27686(0.0000)}    & 29.2   & 1.597    & \textbf{10/10} & \textbf{27686(0.0000)}    & \textbf{27686(0.0000)}      & 172.9  & 0.562   \\
bier127              & 118282               & \textbf{10/10} & \textbf{118282(0.0000)}   & \textbf{118282(0.0000)}   & 1.9    & 0.019    & \textbf{10/10} & \textbf{118282(0.0000)}   & \textbf{118282(0.0000)}     & 1.2    & 0.004   \\
brg180               & 1950                 & \textbf{10/10} & \textbf{1950(0.0000)}     & \textbf{1950(0.0000)}     & 3.9    & 0.006    & \textbf{10/10} & \textbf{1950(0.0000)}     & \textbf{1950(0.0000)}       & 22     & 0.009   \\
ch130                & 6110                 & \textbf{10/10} & \textbf{6110(0.0000)}     & \textbf{6110(0.0000)}     & 4      & 0.017    & \textbf{7/10}  & \textbf{6110(0.0000)}     & \textbf{6114.2(0.0687)}     & 60.7   & 0.017   \\
ch150                & 6528                 & \textbf{10/10} & \textbf{6528(0.0000)}     & \textbf{6528(0.0000)}     & 27.3   & 0.056    & \textbf{7/10}  & \textbf{6528(0.0000)}     & \textbf{6529.5(0.0230)}     & 58.3   & 0.019   \\
d1291                & 50801                & \textbf{10/10} & \textbf{50801(0.0000)}    & \textbf{50801(0.0000)}    & 170.1  & 16.348   & \textbf{0/10}  & \textbf{50803(0.0039)}    & \textbf{50864.1(0.1242)}    & 1291   & 10.175  \\
d1655                & 62128                & \textbf{10/10} & \textbf{62128(0.0000)}    & \textbf{62128(0.0000)}    & 39.3   & 1.108    & \textbf{5/10}  & \textbf{62128(0.0000)}    & \textbf{62138(0.0161)}      & 1102.5 & 3.596   \\
d198                 & 15780                & \textbf{10/10} & \textbf{15780(0.0000)}    & \textbf{15780(0.0000)}    & 18.3   & 0.454    & \textbf{10/10} & \textbf{15780(0.0000)}    & \textbf{15780(0.0000)}      & 30.7   & 0.063   \\
d2103                & 80450                & \textbf{6/10}  & \textbf{80450(0.0000)}    & \textbf{80451.5(0.0019)}  & 945.7  & 474.485  & \textbf{0/10}  & \textbf{80468(0.0224)}    & \textbf{80506.5(0.0702)}    & 2103   & 22.857  \\
d493                 & 35002                & \textbf{10/10} & \textbf{35002(0.0000)}    & \textbf{35002(0.0000)}    & 50.7   & 1.687    & \textbf{0/10}  & \textbf{35004(0.0057)}    & \textbf{35005.9(0.0111)}    & 493    & 1.298   \\
d657                 & 48912                & \textbf{10/10} & \textbf{48912(0.0000)}    & \textbf{48912(0.0000)}    & 25.7   & 0.673    & \textbf{8/10}  & \textbf{48912(0.0000)}    & \textbf{48918.4(0.0131)}    & 247.4  & 0.444   \\
dsj1000              & 18660188             & \textbf{10/10} & \textbf{18660188(0.0000)} & \textbf{18660188(0.0000)} & 31     & 9.069    & \textbf{7/10}  & \textbf{18660188(0.0000)} & \textbf{18666286.7(0.0327)} & 536.7  & 2.697   \\
eil101               & 629                  & \textbf{10/10} & \textbf{629(0.0000)}      & \textbf{629(0.0000)}      & 1      & 0.005    & \textbf{10/10} & \textbf{629(0.0000)}      & \textbf{629(0.0000)}        & 1      & 0.004   \\
fl1400               & 20127                & \textbf{3/10}  & \textbf{20127(0.0000)}    & \textbf{20152.9(0.1287)}  & 1115.4 & 426.471  & 0/10           & \textbf{20164(0.1838)}    & 20195(0.3379)               & 1400   & 27.505  \\
fl1577               & 22249                & \textbf{10/10} & \textbf{22249(0.0000)}    & \textbf{22249(0.0000)}    & 303.5  & 3112.618 & \textbf{0/10}  & \textbf{22263(0.0629)}    & \textbf{22268.6(0.0881)}    & 1577   & 307.747 \\
fl3795               & 28772                & \textbf{4/10}  & \textbf{28772(0.0000)}    & \textbf{28779.8(0.0271)}  & 2590.4 & 2379.836 & \textbf{2/10}  & \textbf{28772(0.0000)}    & \textbf{28788.6(0.0577)}    & 3476.9 & 200.071 \\
fl417                & 11861                & \textbf{10/10} & \textbf{11861(0.0000)}    & \textbf{11861(0.0000)}    & 7.2    & 13.871   & \textbf{10/10} & \textbf{11861(0.0000)}    & \textbf{11861(0.0000)}      & 32.7   & 1.765   \\
fnl4461              & 182566               & \textbf{10/10} & \textbf{182566(0.0000)}   & \textbf{182566(0.0000)}   & 322.4  & 74.652   & \textbf{9/10}  & \textbf{182566(0.0000)}   & \textbf{182566.8(0.0004)}   & 1863.4 & 35.803  \\
gil262               & 2378                 & \textbf{10/10} & \textbf{2378(0.0000)}     & \textbf{2378(0.0000)}     & 7      & 0.247    & \textbf{10/10} & \textbf{2378(0.0000)}     & \textbf{2378(0.0000)}       & 59.7   & 0.123   \\
gr120                & 6942                 & \textbf{10/10} & \textbf{6942(0.0000)}     & \textbf{6942(0.0000)}     & 4.5    & 0.009    & \textbf{8/10}  & \textbf{6942(0.0000)}     & \textbf{6944.8(0.0403)}     & 24.8   & 0.011   \\
gr137                & 69853                & \textbf{9/10}  & \textbf{69853(0.0000)}    & 69865.7(0.0182)           & 14.6   & 0.024    & \textbf{10/10} & \textbf{69853(0.0000)}    & \textbf{69853(0.0000)}      & 1      & 0.006   \\
gr202                & 40160                & \textbf{10/10} & \textbf{40160(0.0000)}    & \textbf{40160(0.0000)}    & 2.4    & 0.029    & \textbf{10/10} & \textbf{40160(0.0000)}    & \textbf{40160(0.0000)}      & 1      & 0.006   \\
gr229                & 134602               & \textbf{10/10} & \textbf{134602(0.0000)}   & \textbf{134602(0.0000)}   & 22     & 0.096    & \textbf{4/10}  & \textbf{134602(0.0000)}   & \textbf{134610.4(0.0062)}   & 158.3  & 0.105   \\
gr431                & 171414               & \textbf{10/10} & \textbf{171414(0.0000)}   & \textbf{171414(0.0000)}   & 107    & 2.997    & \textbf{1/10}  & \textbf{171414(0.0000)}   & \textbf{171522(0.0630)}     & 398.2  & 0.631   \\
gr666                & 294358               & \textbf{7/10}  & \textbf{294358(0.0000)}   & \textbf{294393.4(0.0120)} & 372.4  & 9.903    & \textbf{2/10}  & \textbf{294358(0.0000)}   & \textbf{294452.8(0.0322)}   & 607    & 1.123   \\
kroA150              & 26524                & \textbf{10/10} & \textbf{26524(0.0000)}    & \textbf{26524(0.0000)}    & 2.3    & 0.074    & \textbf{10/10} & \textbf{26524(0.0000)}    & \textbf{26524(0.0000)}      & 26.3   & 0.039   \\
kroA200              & 29368                & \textbf{10/10} & \textbf{29368(0.0000)}    & \textbf{29368(0.0000)}    & 2.5    & 0.156    & \textbf{10/10} & \textbf{29368(0.0000)}    & \textbf{29368(0.0000)}      & 1.5    & 0.023   \\
kroB150              & 26130                & \textbf{8/10}  & \textbf{26130(0.0000)}    & \textbf{26130.4(0.0015)}  & 51.7   & 0.222    & 0/10           & \textbf{26132(0.0077)}    & 26132(0.0077)               & 150    & 0.085   \\
kroB200              & 29437                & \textbf{10/10} & \textbf{29437(0.0000)}    & \textbf{29437(0.0000)}    & 2.1    & 0.067    & \textbf{0/10}  & \textbf{29479(0.1427)}    & \textbf{29479(0.1427)}      & 200    & 0.104   \\
lin105               & 14379                & \textbf{10/10} & \textbf{14379(0.0000)}    & \textbf{14379(0.0000)}    & 1      & 0.002    & \textbf{10/10} & \textbf{14379(0.0000)}    & \textbf{14379(0.0000)}      & 1      & 0.003   \\
lin318               & 42029                & \textbf{8/10}  & \textbf{42029(0.0000)}    & \textbf{42051.8(0.0542)}  & 140.8  & 0.525    & 0/10           & \textbf{42143(0.2712)}    & \textbf{42144.2(0.2741)}    & 318    & 0.117   \\
lin318               & 41345                & \textbf{10/10} & \textbf{41345(0.0000)}    & \textbf{41345(0.0000)}    & 16.7   & 0.087    & \textbf{9/10}  & \textbf{41345(0.0000)}    & \textbf{41349.1(0.0099)}    & 51.8   & 0.029   \\
nrw1379              & 56638                & \textbf{10/10} & \textbf{56638(0.0000)}    & \textbf{56638(0.0000)}    & 476.9  & 23.146   & 4/10           & \textbf{56638(0.0000)}    & \textbf{56641.7(0.0065)}    & 1050.4 & 4.46    \\
p654                 & 34643                & \textbf{10/10} & \textbf{34643(0.0000)}    & \textbf{34643(0.0000)}    & 15.6   & 45.578   & \textbf{8/10}  & \textbf{34643(0.0000)}    & \textbf{34644(0.0029)}      & 201.2  & 10.124  \\
pa561.tsp            & 2763                 & \textbf{10/10} & \textbf{2763(0.0000)}     & \textbf{2763(0.0000)}     & 13.7   & 0.81     & \textbf{10/10} & \textbf{2763(0.0000)}     & \textbf{2763(0.0000)}       & 37.6   & 0.153   \\
pcb1173              & 56892                & \textbf{6/10}  & \textbf{56892(0.0000)}    & \textbf{56894(0.0035)}    & 721.2  & 15.051   & \textbf{3/10}  & \textbf{56892(0.0000)}    & \textbf{56895.5(0.0062)}    & 907.5  & 2.719   \\
pcb3038              & 137694               & \textbf{9/10}  & \textbf{137694(0.0000)}   & \textbf{137694.5(0.0004)} & 1021.9 & 167.493  & \textbf{5/10}  & \textbf{137694(0.0000)}   & \textbf{137706.2(0.0089)}   & 2250.6 & 32.451  \\
pcb442               & 50778                & \textbf{10/10} & \textbf{50778(0.0000)}    & \textbf{50778(0.0000)}    & 4.8    & 0.185    & \textbf{10/10} & \textbf{50778(0.0000)}    & \textbf{50778(0.0000)}      & 11.1   & 0.079   \\
pla7397              & 23260728             & \textbf{10/10} & \textbf{23260728(0.0000)} & \textbf{23260728(0.0000)} & 206.4  & 889.849  & \textbf{7/10}  & \textbf{23260728(0.0000)} & \textbf{23263876(0.0135)}   & 3091.3 & 326.753 \\
pr1002               & 259045               & \textbf{10/10} & \textbf{259045(0.0000)}   & \textbf{259045(0.0000)}   & 281.1  & 4.893    & \textbf{8/10}  & \textbf{259045(0.0000)}   & \textbf{259045.6(0.0002)}   & 711.9  & 1.092   \\
pr107                & 44303                & \textbf{10/10} & \textbf{44303(0.0000)}    & \textbf{44303(0.0000)}    & 1.7    & 0.106    & \textbf{10/10} & \textbf{44303(0.0000)}    & \textbf{44303(0.0000)}      & 1      & 0.008   \\
pr124                & 59030                & \textbf{10/10} & \textbf{59030(0.0000)}    & \textbf{59030(0.0000)}    & 2.2    & 0.03     & \textbf{10/10} & \textbf{59030(0.0000)}    & \textbf{59030(0.0000)}      & 1      & 0.012   \\
pr136                & 96772                & \textbf{10/10} & \textbf{96772(0.0000)}    & \textbf{96772(0.0000)}    & 1.8    & 0.314    & \textbf{10/10} & \textbf{96772(0.0000)}    & \textbf{96772(0.0000)}      & 1      & 0.021   \\
pr144                & 58537                & \textbf{10/10} & \textbf{58537(0.0000)}    & \textbf{58537(0.0000)}    & 2.9    & 0.98     & \textbf{10/10} & \textbf{58537(0.0000)}    & \textbf{58537(0.0000)}      & 1      & 0.048   \\
pr152                & 73682                & \textbf{10/10} & \textbf{73682(0.0000)}    & \textbf{73682(0.0000)}    & 9.7    & 3.531    & \textbf{10/10} & \textbf{73682(0.0000)}    & \textbf{73682(0.0000)}      & 25.8   & 0.05    \\
pr226                & 80369                & \textbf{10/10} & \textbf{80369(0.0000)}    & \textbf{80369(0.0000)}    & 12.4   & 0.591    & \textbf{10/10} & \textbf{80369(0.0000)}    & \textbf{80369(0.0000)}      & 1      & 0.018   \\
pr2392               & 378032               & \textbf{10/10} & \textbf{378032(0.0000)}   & \textbf{378032(0.0000)}   & 13.3   & 42.932   & \textbf{10/10} & \textbf{378032(0.0000)}   & \textbf{378032(0.0000)}     & 114.2  & 12.976  \\
pr299                & 48191                & \textbf{10/10} & \textbf{48191(0.0000)}    & \textbf{48191(0.0000)}    & 3.3    & 0.488    & \textbf{8/10}  & \textbf{48191(0.0000)}    & \textbf{48210.5(0.0405)}    & 144.1  & 0.257   \\
pr439                & 107217               & \textbf{10/10} & \textbf{107217(0.0000)}   & \textbf{107217(0.0000)}   & 65.1   & 1.86     & \textbf{6/10}  & \textbf{107217(0.0000)}   & \textbf{107245.8(0.0269)}   & 276.8  & 0.595   \\
rat195               & 2323                 & \textbf{10/10} & \textbf{2323(0.0000)}     & \textbf{2323(0.0000)}     & 24.7   & 0.285    & \textbf{10/10} & \textbf{2323(0.0000)}     & \textbf{2323(0.0000)}       & 49.1   & 0.072   \\
rat575               & 6773                 & \textbf{7/10}  & \textbf{6773(0.0000)}     & \textbf{6773.4(0.0059)}   & 286.9  & 3.388    & 0/10           & \textbf{6774(0.0148)}     & 6774.1(0.0162)              & 575    & 1.329   \\
rat783               & 8806                 & \textbf{10/10} & \textbf{8806(0.0000)}     & \textbf{8806(0.0000)}     & 18.4   & 0.595    & \textbf{10/10} & \textbf{8806(0.0000)}     & \textbf{8806(0.0000)}       & 64.7   & 0.187   \\
rd400                & 15281                & \textbf{10/10} & \textbf{15281(0.0000)}    & \textbf{15281(0.0000)}    & 34     & 0.534    & \textbf{10/10} & \textbf{15281(0.0000)}    & \textbf{15281(0.0000)}      & 50.1   & 0.141   \\
rl1304               & 252948               & \textbf{8/10}  & \textbf{252948(0.0000)}   & \textbf{252991.3(0.0171)} & 493.4  & 19.742   & \textbf{7/10}  & \textbf{252948(0.0000)}   & \textbf{253045.8(0.0387)}   & 534.1  & 2.036   \\
rl1323               & 270199               & \textbf{9/10}  & \textbf{270199(0.0000)}   & \textbf{270201.7(0.0010)} & 358.2  & 18.002   & \textbf{4/10}  & \textbf{270199(0.0000)}   & \textbf{270303.8(0.0388)}   & 1103.8 & 4.303   \\
rl1889               & 316536               & \textbf{10/10} & \textbf{316536(0.0000)}   & \textbf{316536(0.0000)}   & 420.2  & 91.595   & 0/10           & \textbf{316549(0.0041)}   & 316723(0.0591)              & 1889   & 8.603   \\
rl5915               & 565530               & \textbf{2/10}  & \textbf{565530(0.0000)}   & \textbf{565573.3(0.0077)} & 4927.6 & 1521.327 & \textbf{0/10}  & \textbf{565564(0.0060)}   & \textbf{565701.1(0.0303)}   & 5915   & 124.928 \\
rl5934               & 556045               & \textbf{5/10}  & \textbf{556045(0.0000)}   & \textbf{556130.2(0.0153)} & 4207.3 & 2004.291 & \textbf{0/10}  & \textbf{556225(0.0324)}   & \textbf{556644(0.1077)}     & 5934   & 126.096 \\
si1032               & 92650                & \textbf{10/10} & \textbf{92650(0.0000)}    & \textbf{92650(0.0000)}    & 15.5   & 87.295   & \textbf{10/10} & \textbf{92650(0.0000)}    & \textbf{92650(0.0000)}      & 164.8  & 1.355   \\
si175                & 21407                & \textbf{7/10}  & \textbf{21407(0.0000)}    & \textbf{21407.3(0.0014)}  & 69.2   & 8.273    & \textbf{5/10}  & \textbf{21407(0.0000)}    & \textbf{21407.5(0.0023)}    & 123.4  & 0.492   \\
si535                & 48450                & \textbf{8/10}  & \textbf{48450(0.0000)}    & \textbf{48450.6(0.0012)}  & 192.8  & 77.812   & \textbf{0/10}  & \textbf{48455(0.0103)}    & \textbf{48456.2(0.0128)}    & 535    & 4.403   \\
ts225                & 126643               & \textbf{10/10} & \textbf{126643(0.0000)}   & \textbf{126643(0.0000)}   & 1      & 0.027    & \textbf{10/10} & \textbf{126643(0.0000)}   & \textbf{126643(0.0000)}     & 1      & 0.013   \\
tsp225               & 3916                 & \textbf{10/10} & \textbf{3916(0.0000)}     & \textbf{3916(0.0000)}     & 3.5    & 0.132    & \textbf{10/10} & \textbf{3916(0.0000)}     & \textbf{3916(0.0000)}       & 1.4    & 0.02    \\
u1060                & 224094               & \textbf{10/10} & \textbf{224094(0.0000)}   & \textbf{224094(0.0000)}   & 113.1  & 113.18   & \textbf{5/10}  & \textbf{224094(0.0000)}   & \textbf{224107.5(0.0060)}   & 647.2  & 19.695  \\
u1432                & 152970               & \textbf{10/10} & \textbf{152970(0.0000)}   & \textbf{152970(0.0000)}   & 9.5    & 1.325    & \textbf{10/10} & \textbf{152970(0.0000)}   & \textbf{152970(0.0000)}     & 5.2    & 0.302   \\
u159                 & 42080                & \textbf{10/10} & \textbf{42080(0.0000)}    & \textbf{42080(0.0000)}    & 2.8    & 0.017    & \textbf{10/10} & \textbf{42080(0.0000)}    & \textbf{42080(0.0000)}      & 1      & 0.006   \\
u1817                & 57201                & \textbf{0/10}  & \textbf{57216(0.0262)}    & \textbf{57242.3(0.0722)}  & 1817   & 481.484  & \textbf{0/10}  & \textbf{57256(0.0962)}    & \textbf{57278.8(0.1360)}    & 1817   & 18.862  \\
u2152                & 64253                & \textbf{9/10}  & \textbf{64253(0.0000)}    & \textbf{64257(0.0062)}    & 800.9  & 160.547  & \textbf{3/10}  & \textbf{64253(0.0000)}    & \textbf{64302.4(0.0769)}    & 1680   & 24.841  \\
u2319                & 234256               & \textbf{10/10} & \textbf{234256(0.0000)}   & \textbf{234256(0.0000)}   & 17.8   & 6.453    & \textbf{10/10} & \textbf{234256(0.0000)}   & \textbf{234256(0.0000)}     & 4.1    & 0.595   \\
u574                 & 36905                & \textbf{10/10} & \textbf{36905(0.0000)}    & \textbf{36905(0.0000)}    & 33     & 1.126    & \textbf{8/10}  & \textbf{36905(0.0000)}    & \textbf{36911(0.0163)}      & 204.3  & 0.455   \\
u724                 & 41910                & \textbf{10/10} & \textbf{41910(0.0000)}    & \textbf{41910(0.0000)}    & 90.6   & 3.3      & \textbf{5/10}  & \textbf{41910(0.0000)}    & \textbf{41917.8(0.0186)}    & 564    & 2.651   \\
vm1084               & 239297               & \textbf{8/10}  & \textbf{239297(0.0000)}   & \textbf{239307.4(0.0043)} & 419.8  & 51.722   & \textbf{3/10}  & \textbf{239297(0.0000)}   & \textbf{239416.5(0.0499)}   & 838    & 4.267   \\
vm1748               & 336556               & \textbf{10/10} & \textbf{336556(0.0000)}   & \textbf{336556(0.0000)}   & 257.7  & 18.207   & \textbf{3/10}  & \textbf{336556(0.0000)}   & \textbf{336686(0.0386)}     & 1606.6 & 7.823   \\ \hline
                     & Average Gap(\%)      &                & \textbf{0.0003}           & \textbf{0.0051}           &        &          &                & 0.0115                    & 0.0290                      &        &        \\ \hline
\end{tabular}
}
\caption{Full comparisonal results of \name and \name-$m$ in ablation study. The best results appear in \bf{bold}. }
\label{appendix_$m$}
\end{table*}
\begin{table*}[h]
\centering
\footnotesize
\resizebox{\linewidth}{!}{
\begin{tabular}{rr|rrrrr|rrrrr}
\hline
\multicolumn{1}{l}{} & \multicolumn{1}{l}{} & \multicolumn{5}{c}{\name}                                                   & \multicolumn{5}{c}{\name-$C_{max}$}                                                                                \\
Instance             & BKS                  & Success        & Best(\%)                  & Average(\%)               & Trials & Time(s)  & Success        & Best(\%)                  & Average(\%)               & \multicolumn{1}{r}{Trials} & \multicolumn{1}{r}{Time(s)} \\ \hline
a280                 & 2579                 & \textbf{10/10} & \textbf{2579(0.0000)}     & \textbf{2579(0.0000)}     & 2.4    & 0.025    & \textbf{10/10} & \textbf{2579(0.0000)}     & \textbf{2579(0.0000)}     & 1                          & 0.019                       \\
ali535               & 202339               & \textbf{10/10} & \textbf{202339(0.0000)}   & \textbf{202339(0.0000)}   & 4.2    & 0.325    & \textbf{10/10} & \textbf{202339(0.0000)}   & \textbf{202339(0.0000)}   & 1.6                        & 0.2                         \\
att532               & 27686                & \textbf{10/10} & \textbf{27686(0.0000)}    & \textbf{27686(0.0000)}    & 29.2   & 1.597    & \textbf{10/10} & \textbf{27686(0.0000)}    & \textbf{27686(0.0000)}    & 43.6                       & 1.138                       \\
bier127              & 118282               & \textbf{10/10} & \textbf{118282(0.0000)}   & \textbf{118282(0.0000)}   & 1.9    & 0.019    & \textbf{10/10} & \textbf{118282(0.0000)}   & \textbf{118282(0.0000)}   & 1                          & 0.015                       \\
brg180               & 1950                 & \textbf{10/10} & \textbf{1950(0.0000)}     & \textbf{1950(0.0000)}     & 3.9    & 0.006    & \textbf{10/10} & \textbf{1950(0.0000)}     & \textbf{1950(0.0000)}     & 1.5                        & 0.005                       \\
ch130                & 6110                 & \textbf{10/10} & \textbf{6110(0.0000)}     & \textbf{6110(0.0000)}     & 4      & 0.017    & \textbf{10/10} & \textbf{6110(0.0000)}     & \textbf{6110(0.0000)}     & 1                          & 0.013                       \\
ch150                & 6528                 & \textbf{10/10} & \textbf{6528(0.0000)}     & \textbf{6528(0.0000)}     & 27.3   & 0.056    & \textbf{8/10}  & \textbf{6528(0.0000)}     & \textbf{6529(0.0153)}     & 94                         & 0.188                       \\
d1291                & 50801                & \textbf{10/10} & \textbf{50801(0.0000)}    & \textbf{50801(0.0000)}    & 170.1  & 16.348   & \textbf{10/10} & \textbf{50801(0.0000)}    & \textbf{50801(0.0000)}    & 331.9                      & 40.366                      \\
d1655                & 62128                & \textbf{10/10} & \textbf{62128(0.0000)}    & \textbf{62128(0.0000)}    & 39.3   & 1.108    & \textbf{9/10}  & \textbf{62128(0.0000)}    & \textbf{62128.1(0.0002)}  & 498.8                      & 16.891                      \\
d198                 & 15780                & \textbf{10/10} & \textbf{15780(0.0000)}    & \textbf{15780(0.0000)}    & 18.3   & 0.454    & \textbf{10/10} & \textbf{15780(0.0000)}    & \textbf{15780(0.0000)}    & 8.1                        & 0.428                       \\
d2103                & 80450                & \textbf{6/10}  & \textbf{80450(0.0000)}    & \textbf{80451.5(0.0019)}  & 945.7  & 474.485  & \textbf{3/10}  & \textbf{80450(0.0000)}    & \textbf{80454(0.0050)}    & 1671.6                     & 603.72                      \\
d493                 & 35002                & \textbf{10/10} & \textbf{35002(0.0000)}    & \textbf{35002(0.0000)}    & 50.7   & 1.687    & \textbf{10/10} & \textbf{35002(0.0000)}    & \textbf{35002(0.0000)}    & 18                         & 0.511                       \\
d657                 & 48912                & \textbf{10/10} & \textbf{48912(0.0000)}    & \textbf{48912(0.0000)}    & 25.7   & 0.673    & \textbf{10/10} & \textbf{48912(0.0000)}    & \textbf{48912(0.0000)}    & 40.9                       & 0.694                       \\
dsj1000              & 18660188             & \textbf{10/10} & \textbf{18660188(0.0000)} & \textbf{18660188(0.0000)} & 31     & 9.069    & \textbf{10/10} & \textbf{18660188(0.0000)} & \textbf{18660188(0.0000)} & 176.6                      & 14.678                      \\
eil101               & 629                  & \textbf{10/10} & \textbf{629(0.0000)}      & \textbf{629(0.0000)}      & 1      & 0.005    & \textbf{10/10} & \textbf{629(0.0000)}      & \textbf{629(0.0000)}      & 1                          & 0.004                       \\
fl1400               & 20127                & \textbf{3/10}  & \textbf{20127(0.0000)}    & \textbf{20152.9(0.1287)}  & 1115.4 & 426.471  & \textbf{3/10}  & \textbf{20127(0.0000)}    & \textbf{20152.9(0.1287)}  & 1137.9                     & 596.269                     \\
fl1577               & 22249                & \textbf{10/10} & \textbf{22249(0.0000)}    & \textbf{22249(0.0000)}    & 303.5  & 3112.618 & \textbf{10/10} & \textbf{22249(0.0000)}    & \textbf{22249(0.0000)}    & 233.4                      & 3364.758                    \\
fl3795               & 28772                & \textbf{4/10}  & \textbf{28772(0.0000)}    & \textbf{28779.8(0.0271)}  & 2590.4 & 2379.836 & \textbf{7/10}  & \textbf{28772(0.0000)}    & \textbf{28775.9(0.0136)}  & 2061                       & 2096.536                    \\
fl417                & 11861                & \textbf{10/10} & \textbf{11861(0.0000)}    & \textbf{11861(0.0000)}    & 7.2    & 13.871   & \textbf{10/10} & \textbf{11861(0.0000)}    & \textbf{11861(0.0000)}    & 6.7                        & 29.61                       \\
fnl4461              & 182566               & \textbf{10/10} & \textbf{182566(0.0000)}   & \textbf{182566(0.0000)}   & 322.4  & 74.652   & \textbf{10/10} & \textbf{182566(0.0000)}   & \textbf{182566(0.0000)}   & 1148.9                     & 128.665                     \\
gil262               & 2378                 & \textbf{10/10} & \textbf{2378(0.0000)}     & \textbf{2378(0.0000)}     & 7      & 0.247    & \textbf{10/10} & \textbf{2378(0.0000)}     & \textbf{2378(0.0000)}     & 5.8                        & 0.235                       \\
gr120                & 6942                 & \textbf{10/10} & \textbf{6942(0.0000)}     & \textbf{6942(0.0000)}     & 4.5    & 0.009    & \textbf{10/10} & \textbf{6942(0.0000)}     & \textbf{6942(0.0000)}     & 1                          & 0.01                        \\
gr137                & 69853                & \textbf{9/10}  & \textbf{69853(0.0000)}    & 69865.7(0.0182)           & 14.6   & 0.024    & \textbf{10/10} & \textbf{69853(0.0000)}    & \textbf{69853(0.0000)}    & 1                          & 0.019                       \\
gr202                & 40160                & \textbf{10/10} & \textbf{40160(0.0000)}    & \textbf{40160(0.0000)}    & 2.4    & 0.029    & \textbf{10/10} & \textbf{40160(0.0000)}    & \textbf{40160(0.0000)}    & 1.5                        & 0.022                       \\
gr229                & 134602               & \textbf{10/10} & \textbf{134602(0.0000)}   & \textbf{134602(0.0000)}   & 22     & 0.096    & \textbf{10/10} & \textbf{134602(0.0000)}   & \textbf{134602(0.0000)}   & 19                         & 0.103                       \\
gr431                & 171414               & \textbf{10/10} & \textbf{171414(0.0000)}   & \textbf{171414(0.0000)}   & 107    & 2.997    & \textbf{10/10} & \textbf{171414(0.0000)}   & \textbf{171414(0.0000)}   & 163.4                      & 3.709                       \\
gr666                & 294358               & \textbf{7/10}  & \textbf{294358(0.0000)}   & \textbf{294393.4(0.0120)} & 372.4  & 9.903    & \textbf{4/10}  & \textbf{294358(0.0000)}   & \textbf{294428.8(0.0241)} & 444.1                      & 8.923                       \\
kroA150              & 26524                & \textbf{10/10} & \textbf{26524(0.0000)}    & \textbf{26524(0.0000)}    & 2.3    & 0.074    & \textbf{10/10} & \textbf{26524(0.0000)}    & \textbf{26524(0.0000)}    & 1                          & 0.067                       \\
kroA200              & 29368                & \textbf{10/10} & \textbf{29368(0.0000)}    & \textbf{29368(0.0000)}    & 2.5    & 0.156    & \textbf{10/10} & \textbf{29368(0.0000)}    & \textbf{29368(0.0000)}    & 1                          & 0.125                       \\
kroB150              & 26130                & \textbf{8/10}  & \textbf{26130(0.0000)}    & \textbf{26130.4(0.0015)}  & 51.7   & 0.222    & \textbf{9/10}  & \textbf{26130(0.0000)}    & \textbf{26130.2(0.0008)}  & 77                         & 0.547                       \\
kroB200              & 29437                & \textbf{10/10} & \textbf{29437(0.0000)}    & \textbf{29437(0.0000)}    & 2.1    & 0.067    & \textbf{10/10} & \textbf{29437(0.0000)}    & \textbf{29437(0.0000)}    & 1                          & 0.053                       \\
lin105               & 14379                & \textbf{10/10} & \textbf{14379(0.0000)}    & \textbf{14379(0.0000)}    & 1      & 0.002    & \textbf{10/10} & \textbf{14379(0.0000)}    & \textbf{14379(0.0000)}    & 1                          & 0.002                       \\
lin318               & 42029                & \textbf{8/10}  & \textbf{42029(0.0000)}    & \textbf{42051.8(0.0542)}  & 140.8  & 0.525    & \textbf{8/10}  & \textbf{42029(0.0000)}    & \textbf{42051.8(0.0542)}  & 98.4                       & 0.797                       \\
lin318               & 41345                & \textbf{10/10} & \textbf{41345(0.0000)}    & \textbf{41345(0.0000)}    & 16.7   & 0.087    & \textbf{10/10} & \textbf{41345(0.0000)}    & \textbf{41345(0.0000)}    & 1.8                        & 0.04                        \\
nrw1379              & 56638                & \textbf{10/10} & \textbf{56638(0.0000)}    & \textbf{56638(0.0000)}    & 476.9  & 23.146   & 7/10           & \textbf{56638(0.0000)}    & \textbf{56639.5(0.0026)}  & 662.7                      & 21.268                      \\
p654                 & 34643                & \textbf{10/10} & \textbf{34643(0.0000)}    & \textbf{34643(0.0000)}    & 15.6   & 45.578   & \textbf{10/10} & \textbf{34643(0.0000)}    & \textbf{34643(0.0000)}    & 8.4                        & 37.885                      \\
pa561.tsp            & 2763                 & \textbf{10/10} & \textbf{2763(0.0000)}     & \textbf{2763(0.0000)}     & 13.7   & 0.81     & \textbf{10/10} & \textbf{2763(0.0000)}     & \textbf{2763(0.0000)}     & 14.1                       & 0.536                       \\
pcb1173              & 56892                & \textbf{6/10}  & \textbf{56892(0.0000)}    & \textbf{56894(0.0035)}    & 721.2  & 15.051   & \textbf{7/10}  & \textbf{56892(0.0000)}    & \textbf{56893.5(0.0026)}  & 693.3                      & 12.284                      \\
pcb3038              & 137694               & \textbf{9/10}  & \textbf{137694(0.0000)}   & \textbf{137694.5(0.0004)} & 1021.9 & 167.493  & \textbf{8/10}  & \textbf{137694(0.0000)}   & \textbf{137695(0.0007)}   & 1416.8                     & 153.765                     \\
pcb442               & 50778                & \textbf{10/10} & \textbf{50778(0.0000)}    & \textbf{50778(0.0000)}    & 4.8    & 0.185    & \textbf{10/10} & \textbf{50778(0.0000)}    & \textbf{50778(0.0000)}    & 6.4                        & 0.305                       \\
pla7397              & 23260728             & \textbf{10/10} & \textbf{23260728(0.0000)} & \textbf{23260728(0.0000)} & 206.4  & 889.849  & \textbf{10/10} & \textbf{23260728(0.0000)} & \textbf{23260728(0.0000)} & 406.9                      & 973.072                     \\
pr1002               & 259045               & \textbf{10/10} & \textbf{259045(0.0000)}   & \textbf{259045(0.0000)}   & 281.1  & 4.893    & \textbf{6/10}  & \textbf{259045(0.0000)}   & \textbf{259046.5(0.0006)} & 645.5                      & 6.626                       \\
pr107                & 44303                & \textbf{10/10} & \textbf{44303(0.0000)}    & \textbf{44303(0.0000)}    & 1.7    & 0.106    & \textbf{10/10} & \textbf{44303(0.0000)}    & \textbf{44303(0.0000)}    & 1                          & 0.642                       \\
pr124                & 59030                & \textbf{10/10} & \textbf{59030(0.0000)}    & \textbf{59030(0.0000)}    & 2.2    & 0.03     & \textbf{10/10} & \textbf{59030(0.0000)}    & \textbf{59030(0.0000)}    & 1                          & 0.209                       \\
pr136                & 96772                & \textbf{10/10} & \textbf{96772(0.0000)}    & \textbf{96772(0.0000)}    & 1.8    & 0.314    & \textbf{10/10} & \textbf{96772(0.0000)}    & \textbf{96772(0.0000)}    & 1                          & 0.323                       \\
pr144                & 58537                & \textbf{10/10} & \textbf{58537(0.0000)}    & \textbf{58537(0.0000)}    & 2.9    & 0.98     & \textbf{10/10} & \textbf{58537(0.0000)}    & \textbf{58537(0.0000)}    & 1                          & 1.756                       \\
pr152                & 73682                & \textbf{10/10} & \textbf{73682(0.0000)}    & \textbf{73682(0.0000)}    & 9.7    & 3.531    & \textbf{10/10} & \textbf{73682(0.0000)}    & \textbf{73682(0.0000)}    & 9.7                        & 7.943                       \\
pr226                & 80369                & \textbf{10/10} & \textbf{80369(0.0000)}    & \textbf{80369(0.0000)}    & 12.4   & 0.591    & \textbf{10/10} & \textbf{80369(0.0000)}    & \textbf{80369(0.0000)}    & 1                          & 0.53                        \\
pr2392               & 378032               & \textbf{10/10} & \textbf{378032(0.0000)}   & \textbf{378032(0.0000)}   & 13.3   & 42.932   & \textbf{10/10} & \textbf{378032(0.0000)}   & \textbf{378032(0.0000)}   & 15.9                       & 28.087                      \\
pr299                & 48191                & \textbf{10/10} & \textbf{48191(0.0000)}    & \textbf{48191(0.0000)}    & 3.3    & 0.488    & \textbf{10/10} & \textbf{48191(0.0000)}    & \textbf{48191(0.0000)}    & 1                          & 0.459                       \\
pr439                & 107217               & \textbf{10/10} & \textbf{107217(0.0000)}   & \textbf{107217(0.0000)}   & 65.1   & 1.86     & \textbf{9/10}  & \textbf{107217(0.0000)}   & \textbf{107224.2(0.0067)} & 81.6                       & 3.385                       \\
rat195               & 2323                 & \textbf{10/10} & \textbf{2323(0.0000)}     & \textbf{2323(0.0000)}     & 24.7   & 0.285    & \textbf{10/10} & \textbf{2323(0.0000)}     & \textbf{2323(0.0000)}     & 3                          & 0.171                       \\
rat575               & 6773                 & \textbf{7/10}  & \textbf{6773(0.0000)}     & \textbf{6773.4(0.0059)}   & 286.9  & 3.388    & 4/10           & \textbf{6773(0.0000)}     & 6773.6(0.0089)            & 407.4                      & 4.873                       \\
rat783               & 8806                 & \textbf{10/10} & \textbf{8806(0.0000)}     & \textbf{8806(0.0000)}     & 18.4   & 0.595    & \textbf{10/10} & \textbf{8806(0.0000)}     & \textbf{8806(0.0000)}     & 23.6                       & 0.63                        \\
rd400                & 15281                & \textbf{10/10} & \textbf{15281(0.0000)}    & \textbf{15281(0.0000)}    & 34     & 0.534    & \textbf{10/10} & \textbf{15281(0.0000)}    & \textbf{15281(0.0000)}    & 4.3                        & 0.261                       \\
rl1304               & 252948               & \textbf{8/10}  & \textbf{252948(0.0000)}   & \textbf{252991.3(0.0171)} & 493.4  & 19.742   & \textbf{7/10}  & \textbf{252948(0.0000)}   & \textbf{252993(0.0178)}   & 615.4                      & 37.54                       \\
rl1323               & 270199               & \textbf{9/10}  & \textbf{270199(0.0000)}   & \textbf{270201.7(0.0010)} & 358.2  & 18.002   & \textbf{9/10}  & \textbf{270199(0.0000)}   & \textbf{270201.7(0.0010)} & 481                        & 33.021                      \\
rl1889               & 316536               & \textbf{10/10} & \textbf{316536(0.0000)}   & \textbf{316536(0.0000)}   & 420.2  & 91.595   & \textbf{10/10} & \textbf{316536(0.0000)}   & \textbf{316536(0.0000)}   & 440.4                      & 82.657                      \\
rl5915               & 565530               & \textbf{2/10}  & \textbf{565530(0.0000)}   & \textbf{565573.3(0.0077)} & 4927.6 & 1521.327 & \textbf{0/10}  & \textbf{565585(0.0097)}   & \textbf{565591.7(0.0109)} & 5915                       & 758.785                     \\
rl5934               & 556045               & \textbf{5/10}  & \textbf{556045(0.0000)}   & \textbf{556130.2(0.0153)} & 4207.3 & 2004.291 & \textbf{1/10}  & \textbf{556045(0.0000)}   & \textbf{556280.9(0.0424)} & 5422                       & 1123.201                    \\
si1032               & 92650                & \textbf{10/10} & \textbf{92650(0.0000)}    & \textbf{92650(0.0000)}    & 15.5   & 87.295   & \textbf{10/10} & \textbf{92650(0.0000)}    & \textbf{92650(0.0000)}    & 16.2                       & 139.862                     \\
si175                & 21407                & \textbf{7/10}  & \textbf{21407(0.0000)}    & \textbf{21407.3(0.0014)}  & 69.2   & 8.273    & \textbf{10/10} & \textbf{21407(0.0000)}    & \textbf{21407(0.0000)}    & 38.9                       & 17.281                      \\
si535                & 48450                & \textbf{8/10}  & \textbf{48450(0.0000)}    & \textbf{48450.6(0.0012)}  & 192.8  & 77.812   & \textbf{8/10}  & \textbf{48450(0.0000)}    & \textbf{48450.6(0.0012)}  & 231.1                      & 229.39                      \\
ts225                & 126643               & \textbf{10/10} & \textbf{126643(0.0000)}   & \textbf{126643(0.0000)}   & 1      & 0.027    & \textbf{10/10} & \textbf{126643(0.0000)}   & \textbf{126643(0.0000)}   & 1                          & 0.096                       \\
tsp225               & 3916                 & \textbf{10/10} & \textbf{3916(0.0000)}     & \textbf{3916(0.0000)}     & 3.5    & 0.132    & \textbf{10/10} & \textbf{3916(0.0000)}     & \textbf{3916(0.0000)}     & 1.2                        & 0.154                       \\
u1060                & 224094               & \textbf{10/10} & \textbf{224094(0.0000)}   & \textbf{224094(0.0000)}   & 113.1  & 113.18   & \textbf{10/10} & \textbf{224094(0.0000)}   & \textbf{224094(0.0000)}   & 22.1                       & 28.136                      \\
u1432                & 152970               & \textbf{10/10} & \textbf{152970(0.0000)}   & \textbf{152970(0.0000)}   & 9.5    & 1.325    & \textbf{10/10} & \textbf{152970(0.0000)}   & \textbf{152970(0.0000)}   & 4.4                        & 2.31                        \\
u159                 & 42080                & \textbf{10/10} & \textbf{42080(0.0000)}    & \textbf{42080(0.0000)}    & 2.8    & 0.017    & \textbf{10/10} & \textbf{42080(0.0000)}    & \textbf{42080(0.0000)}    & 1                          & 0.019                       \\
u1817                & 57201                & \textbf{0/10}  & \textbf{57216(0.0262)}    & \textbf{57242.3(0.0722)}  & 1817   & 481.484  & \textbf{1/10}  & \textbf{57201(0.0000)}    & \textbf{57229.3(0.0495)}  & 1783.2                     & 476.549                     \\
u2152                & 64253                & \textbf{9/10}  & \textbf{64253(0.0000)}    & \textbf{64257(0.0062)}    & 800.9  & 160.547  & \textbf{7/10}  & \textbf{64253(0.0000)}    & \textbf{64270.1(0.0266)}  & 879.8                      & 236.826                     \\
u2319                & 234256               & \textbf{10/10} & \textbf{234256(0.0000)}   & \textbf{234256(0.0000)}   & 17.8   & 6.453    & \textbf{10/10} & \textbf{234256(0.0000)}   & \textbf{234256(0.0000)}   & 3.8                        & 2.957                       \\
u574                 & 36905                & \textbf{10/10} & \textbf{36905(0.0000)}    & \textbf{36905(0.0000)}    & 33     & 1.126    & \textbf{10/10} & \textbf{36905(0.0000)}    & \textbf{36905(0.0000)}    & 3                          & 0.485                       \\
u724                 & 41910                & \textbf{10/10} & \textbf{41910(0.0000)}    & \textbf{41910(0.0000)}    & 90.6   & 3.3      & \textbf{10/10} & \textbf{41910(0.0000)}    & \textbf{41910(0.0000)}    & 68.7                       & 2.205                       \\
vm1084               & 239297               & \textbf{8/10}  & \textbf{239297(0.0000)}   & \textbf{239307.4(0.0043)} & 419.8  & 51.722   & \textbf{6/10}  & \textbf{239297(0.0000)}   & \textbf{239334.4(0.0156)} & 512.1                      & 75.545                      \\
vm1748               & 336556               & \textbf{10/10} & \textbf{336556(0.0000)}   & \textbf{336556(0.0000)}   & 257.7  & 18.207   & \textbf{9/10}  & \textbf{336556(0.0000)}   & \textbf{336556.4(0.0001)} & 743.1                      & 43.639                      \\ \hline
                     & Average Gap(\%)      &                & 0.0003           & \textbf{0.0051}           &        &          &                & \textbf{0.0001}           & 0.0057                    & \multicolumn{1}{r}{}       & \multicolumn{1}{r}{}       \\ \hline
\end{tabular}
}
\caption{Full comparisonal results of \name and \name-$C_{max}$ in ablation study. The best results appear in \bf{bold}. }
\label{appendix_cmax}
\end{table*}

% 分析一下
In table \ref{appendix_$m$} and \ref{appendix_cmax}, \name has best performance among three experiments overall, which shows $\alpha$ is not good enough for algorithm to provide superior candidate edges while the magical design of combining MAB models with candidate edges could find more fancy edges, providing more guidance information and enhancing the search capability of LKH.

\subsection{Supplement of Generalization Evaluation}
MTSP is a classical variance of TSP and can be solved by LKH3, in which involving multiple salesmen, each tasked with visiting a subset of cities while adhering to specific constraints, with the objective of minimizing the total travel cost or time. Instances in MTSP are good test benchmark for algorithm. Therefore, we extend \name to the framework of LKH3 to indicate good generalization property of our proposed method.

\begin{table*}[h]
\centering
\footnotesize
% \resizebox{\linewidth}{!}{
\begin{tabular}{r|rrr|rrr}
\hline
\multicolumn{1}{l}{} & \multicolumn{3}{c}{LKH3}                           & \multicolumn{3}{c}{Band-LKH3}                        \\
Instance                 & Best               & Average               & Time(s) & Best                & Average                  & Time(s)     \\ \hline
a280                 & \textbf{2645}     & \textbf{2645}     & 0.009      & \textbf{2645}      & 2656.5               & 0.02     \\
ali535               & 203472            & 205287            & 0.114      & \textbf{203044}    & \textbf{204406.8}    & 0.137    \\
att48                & \textbf{11014}    & \textbf{11014}    & 0.001      & \textbf{11014}     & \textbf{11014}       & 0.001    \\
att532               & \textbf{28310}    & 28354             & 0.096      & 28323              & \textbf{28340.2}     & 0.105    \\
bayg29               & \textbf{1718}     & \textbf{1718}     & 0          & \textbf{1718}      & \textbf{1718}        & 0        \\
bays29               & \textbf{2139}     & \textbf{2139}     & 0.001      & \textbf{2139}      & \textbf{2139}        & 0        \\
berlin52             & \textbf{7735}     & \textbf{7735}     & 0.001      & \textbf{7735}      & \textbf{7735}        & 0        \\
bier127              & \textbf{119163}   & \textbf{119163}   & 0.004      & \textbf{119163}    & \textbf{119163}      & 0.003    \\
brazil58             & \textbf{26538}    & \textbf{26538}    & 0.002      & \textbf{26538}     & \textbf{26538}       & 0.001    \\
brd14051             & 478611            & 483402.6          & 27.828     & \textbf{474936}    & \textbf{475305.2}    & 78.244   \\
brg180               & \textbf{1980}     & \textbf{1980}     & 0.003      & \textbf{1980}      & \textbf{1980}        & 0.005    \\
burma14              & \textbf{3547}     & \textbf{3547}     & 0          & \textbf{3547}      & \textbf{3547}        & 0        \\
ch130                & \textbf{6296}     & \textbf{6296}     & 0.005      & \textbf{6296}      & \textbf{6296}        & 0.005    \\
ch150                & \textbf{6571}     & \textbf{6589.67}  & 0.02       & \textbf{6571}      & \textbf{6571}        & 0.006    \\
d1291                & \textbf{56320}    & \textbf{56390.6}  & 0.244      & 56541              & 56819.4              & 0.308    \\
d15112               & 1604194           & 1604374.8         & 32.079     & \textbf{1593905}   & \textbf{1594424.8}   & 111.195  \\
d1655                & \textbf{68582}    & \textbf{68937.4}  & 0.392      & 68826              & 69305.2              & 0.528    \\
d18512               & 658656            & 659308            & 49.862     & \textbf{654037}    & \textbf{654150.8}    & 116.807  \\
d198                 & \textbf{20351}    & \textbf{20351}    & 0.009      & \textbf{20351}     & \textbf{20351.5}     & 0.023    \\
d2103                & 85852             & 86378.6           & 0.486      & \textbf{85786}     & \textbf{86333.6}     & 0.604    \\
d493                 & 42785             & 42876.6           & 0.098      & \textbf{42753}     & \textbf{42790}       & 0.113    \\
d657                 & 54422             & 54697.8           & 0.105      & \textbf{54396}     & \textbf{54521.4}     & 0.125    \\
dantzig42            & \textbf{703}      & \textbf{703}      & 0.001      & \textbf{703}       & \textbf{703}         & 0.001    \\
dsj1000              & \textbf{18780343} & 18840808.2        & 0.215      & 18809451           & \textbf{18830484.2}  & 0.286    \\
eil101               & \textbf{646}      & \textbf{646}      & 0.004      & \textbf{646}       & \textbf{646}         & 0.004    \\
eil51                & \textbf{443}      & \textbf{443}      & 0.001      & \textbf{443}       & \textbf{443}         & 0.002    \\
eil76                & \textbf{555}      & \textbf{555}      & 0.002      & \textbf{555}       & \textbf{555}         & 0.002    \\
fl1400               & 21294             & 21515.4           & 0.41       & \textbf{21094}     & \textbf{21119.6}     & 0.575    \\
fl1577               & \textbf{22574}    & 23266.8           & 0.341      & 22603              & \textbf{22943}       & 0.428    \\
fl3795               & \textbf{33249}    & 33496             & 1.621      & 32305              & \textbf{32902.4}     & 2.279    \\
fl417                & \textbf{11941}    & 12065.33          & 0.051      & \textbf{11941}     & \textbf{11941.67}    & 0.079    \\
fnl4461              & 185381            & 186091.4          & 2.657      & \textbf{184933}    & \textbf{185112.6}    & 4.094    \\
fri26                & \textbf{1214}     & \textbf{1214}     & 0.001      & \textbf{1214}      & \textbf{1214}        & 0        \\
gil262               & \textbf{2447}     & \textbf{2453.8}   & 0.044      & \textbf{2447}      & \textbf{2450}        & 0.058    \\
gr120                & \textbf{7196}     & \textbf{7196}     & 0.003      & \textbf{7196}      & \textbf{7196}        & 0.008    \\
gr137                & \textbf{73410}    & \textbf{73410}    & 0.004      & \textbf{73410}     & \textbf{73410}       & 0.004    \\
gr17                 & \textbf{2322}     & \textbf{2322}     & 0          & \textbf{2322}      & \textbf{2322}        & 0        \\
gr202                & \textbf{45838}    & \textbf{45851.5}  & 0.018      & \textbf{45838}     & \textbf{45851.5}     & 0.02     \\
gr21                 & \textbf{3022}     & \textbf{3022}     & 0          & \textbf{3022}      & \textbf{3022}        & 0        \\
gr229                & 137521            & 137935            & 0.057      & \textbf{137357}    & \textbf{137780}      & 0.07     \\
gr24                 & \textbf{1523}     & \textbf{1523}     & 0.001      & \textbf{1523}      & \textbf{1523}        & 0        \\
gr431                & 177596            & 177854.2          & 0.083      & \textbf{177336}    & \textbf{177643}      & 0.1      \\
gr48                 & \textbf{5333}     & \textbf{5333}     & 0.001      & \textbf{5333}      & \textbf{5333}        & 0.002    \\
gr666                & \textbf{300910}   & \textbf{301704.8} & 0.118      & 301747             & 302599.4             & 0.142    \\
gr96                 & \textbf{57922}    & \textbf{57922}    & 0.002      & \textbf{57922}     & \textbf{57922}       & 0.003    \\
hk48                 & \textbf{12107}    & \textbf{12107}    & 0.001      & \textbf{12107}     & \textbf{12107}       & 0.001    \\
kroA100              & \textbf{22059}    & \textbf{22059}    & 0.002      & \textbf{22059}     & \textbf{22059}       & 0.002    \\
kroA150              & \textbf{26943}    & \textbf{26943}    & 0.003      & \textbf{26943}     & \textbf{26943}       & 0.004    \\
kroA200              & \textbf{29538}    & \textbf{29547.33} & 0.024      & 29552              & 29552                & 0.054    \\
kroB100              & \textbf{22472}    & \textbf{22472}    & 0.003      & \textbf{22472}     & \textbf{22472}       & 0.009    \\
kroB150              & \textbf{26476}    & \textbf{26476}    & 0.008      & \textbf{26476}     & \textbf{26476}       & 0.013    \\
kroB200              & \textbf{29767}    & \textbf{29767}    & 0.005      & \textbf{29767}     & 29788.75             & 0.041    \\
kroC100              & \textbf{21212}    & \textbf{21212}    & 0.002      & \textbf{21212}     & \textbf{21212}       & 0.002    \\
kroD100              & \textbf{21796}    & \textbf{21796}    & 0.002      & \textbf{21796}     & \textbf{21796}       & 0.001    \\
kroE100              & \textbf{22348}    & \textbf{22348}    & 0.004      & \textbf{22348}     & \textbf{22348}       & 0.002    \\
lin105               & \textbf{14741}    & \textbf{14741}    & 0.002      & \textbf{14741}     & \textbf{14741}       & 0.002    \\
lin318               & \textbf{42391}    & \textbf{42478}    & 0.025      & 42412              & 42548.8              & 0.066    \\
linhp318             & \textbf{41711}    & \textbf{41768.2}  & 0.053      & 41748              & 41849                & 0.071    \\
nrw1379              & 57099             & 57207.4           & 0.292      & \textbf{57001}     & \textbf{57165.2}     & 0.414    \\
p654                 & \textbf{36890}    & 37413.6           & 0.134      & \textbf{36890}     & \textbf{36897.67}    & 0.101    \\
pa561                & 2817              & 2819.8            & 0.115      & \textbf{2806}      & \textbf{2812.6}      & 0.13     \\
pcb1173              & 57880             & 57942             & 0.213      & \textbf{57660}     & \textbf{57861.4}     & 0.275    \\
pcb3038              & \textbf{140077}   & \textbf{140308.2} & 1.128      & 140125             & 140322.6             & 1.413    \\
pcb442               & \textbf{51071}    & 51137             & 0.072      & 51094              & 51318.4              & 0.083    \\
pla33810             & 70686837          & 70769236.6        & 177.446    & \textbf{68567400}  & \textbf{68808980.6}  & 391.441  \\
pla7397              & 24404268          & 24607606.6        & 6.64       & \textbf{23928458}  & \textbf{23991798.4}  & 11.326   \\
pla85900             & 166383078         & 166720326.8       & 2042.296   & \textbf{157305820} & \textbf{158179771.8} & 2769.294 \\
pr1002               & \textbf{264134}   & \textbf{265246.4} & 0.178      & 265713             & 266412               & 0.216    \\
pr107                & \textbf{44869}    & \textbf{44869}    & 0.003      & \textbf{44869}     & \textbf{44869}       & 0.004    \\
pr124                & \textbf{59979}    & \textbf{59979}    & 0.003      & \textbf{59979}     & \textbf{59979}       & 0.002    \\
pr136                & \textbf{98629}    & \textbf{98740}    & 0.019      & \textbf{98629}     & \textbf{98629}       & 0.01     \\ \hline
\end{tabular}
% }
\caption{The first part of full comparisonal results of LKH and \name in mTSP. The best results appear in \bf{bold}. }
\label{appendix_mTSP1}
\end{table*}
\begin{table*}[h]
\centering
\footnotesize
\resizebox{\linewidth}{!}{
\begin{tabular}{r|rrr|rrr}
\hline
\multicolumn{1}{l}{} & \multicolumn{3}{c}{LKH3}                         & \multicolumn{3}{c}{Band-LKH3}                    \\ 
Instance                 & Best             & Average               & Time(s) & Best               & Average                 & Time(s)   \\ \hline
pr144                & \textbf{59444}    & \textbf{59444}    & 0.003      & \textbf{59444}     & \textbf{59444}       & 0.004    \\ 
pr152                & \textbf{75893}  & \textbf{75893}    & 0.006      & \textbf{75893}    & \textbf{75893}      & 0.007  \\
pr226                & \textbf{84109}  & \textbf{84144.5}  & 0.014      & \textbf{84109}    & \textbf{84109}      & 0.008  \\
pr2392               & 384311          & 386713            & 0.693      & \textbf{383045}   & \textbf{384996.6}   & 0.883  \\
pr264                & 49947           & 50010.4           & 0.037      & \textbf{49704}    & \textbf{49738}      & 0.02   \\
pr299                & \textbf{48821}  & \textbf{49071.8}  & 0.057      & 48889             & 49000.6             & 0.074  \\
pr439                & \textbf{108126} & 109305.2          & 0.068      & \textbf{108126}   & \textbf{108989.2}   & 0.089  \\
pr76                 & \textbf{111056} & \textbf{111056}   & 0.004      & \textbf{111056}   & \textbf{111056}     & 0.003  \\
rat195               & \textbf{2381}   & \textbf{2385.33}  & 0.023      & \textbf{2381}     & 2385.8              & 0.045  \\
rat575               & \textbf{6821}   & \textbf{6850.6}   & 0.087      & 6832              & \textbf{6850.6}     & 0.105  \\
rat783               & 8902            & 8916.2            & 0.126      & \textbf{8873}     & \textbf{8906}       & 0.156  \\
rat99                & \textbf{1269}   & \textbf{1269}     & 0.004      & \textbf{1269}     & \textbf{1269}       & 0.003  \\
rd100                & \textbf{8012}   & \textbf{8012}     & 0.005      & \textbf{8012}     & \textbf{8012}       & 0.003  \\
rd400                & \textbf{15355}  & \textbf{15391.6}  & 0.066      & 15366             & 15395.2             & 0.075  \\
rl11849              & 998816          & 1007830.4         & 18.115     & \textbf{940468}   & \textbf{942182}     & 50.34  \\
rl1304               & 257894          & 262147            & 0.262      & \textbf{254936}   & \textbf{255536.4}   & 0.34   \\
rl1323               & 274672          & 278159.6          & 0.259      & \textbf{273005}   & \textbf{274332.8}   & 0.338  \\
rl1889               & 324006          & \textbf{324944.2} & 0.504      & \textbf{320878}   & 325690.8            & 0.675  \\
rl5915               & 599265          & 601361            & 4.108      & \textbf{587629}   & \textbf{590227.6}   & 7.201  \\
rl5934               & 593816          & 597851.4          & 4.121      & \textbf{571066}   & \textbf{586723.2}   & 5.814  \\
si1032               & 93045           & 93101.2           & 0.187      & \textbf{92959}    & \textbf{93025}      & 0.231  \\
si175                & \textbf{21717}  & 21725.4           & 0.047      & \textbf{21717}    & \textbf{21723.5}    & 0.019  \\
si535                & 48914           & 48966             & 0.1        & \textbf{48907}    & \textbf{48916.2}    & 0.129  \\
st70                 & \textbf{689}    & \textbf{689}      & 0.004      & \textbf{689}      & \textbf{689}        & 0.001  \\
swiss42              & \textbf{1333}   & \textbf{1333}     & 0.001      & \textbf{1333}     & \textbf{1333}       & 0.001  \\
ts225                & \textbf{128643} & \textbf{128643}   & 0.006      & \textbf{128643}   & \textbf{128643}     & 0.007  \\
tsp225               & \textbf{3988}   & \textbf{4009.67}  & 0.025      & \textbf{3988}     & \textbf{3988}       & 0.012  \\
u1060                & \textbf{225648} & 226778.4          & 0.219      & 225759            & \textbf{226196.4}   & 0.276  \\
u1432                & 154056          & 154629.2          & 0.323      & \textbf{154319}   & \textbf{154480}     & 0.413  \\
u159                 & \textbf{43846}  & \textbf{43846}    & 0.003      & \textbf{43846}    & \textbf{43846}      & 0.003  \\
u1817                & 58222           & 58310             & 0.44       & \textbf{58120}    & \textbf{58307}      & 0.546  \\
u2152                & \textbf{65025}  & \textbf{65179.2}  & 0.606      & 65410             & 65660               & 0.822  \\
u2319                & \textbf{235352} & \textbf{235563.8} & 0.715      & 235779            & 235879.2            & 0.901  \\
u574                 & \textbf{37012}  & \textbf{37113}    & 0.086      & 37030             & 37168               & 0.11   \\
u724                 & \textbf{42599}  & 42788.8           & 0.117      & 42719             & \textbf{42784.8}    & 0.139  \\
ulysses16            & \textbf{7112}   & \textbf{7112}     & 0          & \textbf{7112}     & \textbf{7112}       & 0      \\
ulysses22            & \textbf{7259}   & \textbf{7259}     & 0          & \textbf{7259}     & \textbf{7259}       & 0      \\
usa13509             & 20785341        & 21020059          & 24.693     & \textbf{20252999} & \textbf{20329103.6} & 66.721 \\
vm1084               & \textbf{241570} & \textbf{242288.2} & 0.209      & 242063            & 242842              & 0.274  \\ 
vm1748               & 343521          & 344526.4          & 0.464      & \textbf{341308}   & \textbf{342488}     & 0.635 \\ \hline
\end{tabular}
}
\caption{The second part of full comparisonal results of LKH and \name in mTSP. The best results appear in \bf{bold}. }
\label{appendix_mtsp2}
\end{table*}
% 这里讲我们测试了多少算例，算例的大概
% 总的结果，结论
We test 111 instances in TSPLIB and show the results in table \ref{appendix_mTSP1} and \ref{appendix_mtsp2}. Among 82 big instances, \name obtains a better result than LKH in 33 (resp. 47) instances in terms of the best (resp. average) solutions and a worse result than LKH in 21 (resp. 19) instances in terms of the best (resp. average) solutions. \name performed well in many instances, such as ali535, rl5934, brd14051, d18512, pla33810, pla85900 and so on. In other 29 instances, two algorithms achieve the same outcome.

The outcome of generalization evaluation shows that \name could be extended to perfect framework for other variant problem and achieve better performance, which indicates our method has good performance and generalization.
